# Supplementary material for: A spectral clustering approach for the evolution of the COVID-19 pandemic in the state of Rio Grande do Sul, Brazil
Source: arXiv:2008.00333 ancillary file (2020-08-04)
Supplement: Supplementary file 1 [file A_spectral_clustering_approach_for_the_evolution_of_the_COVID-19_pandemic_in_the_state_of_Rio_Grande_do_Sul,_Brazil_-_Graphs.pdf]

---

# A spectral clustering approach for the evolution of the COVID-19 pandemic in the state of Rio Grande do Sul, Brazil

Luiz Emilio Allem<sup>1</sup>, Carlos Hoppen<sup>2</sup>, Matheus Micadei Marzo<sup>3</sup>, Lucas Siviero Sibemberg<sup>4</sup>

Instituto de Matemática e Estatística, Universidade Federal do Rio Grande do Sul, Av. Bento Gonçalves, 9500, 91509-900, Porto Alegre, RS, Brasil.

**Abstract.** This file complements the paper of the same title. Regarding pendulum migration, we describe the dissemination of COVID-19 within each cluster. Regarding ICU beds, we give information about all clusterings. Regarding our SEIR model, we show the results of our simulations in several cities.

---

<sup>1</sup>emilio.allem@ufrgs.br.

<sup>2</sup>choppen@ufrgs.br.

<sup>3</sup>matheus.marzo@ufrgs.br.

<sup>4</sup>lucas.siviero@ufrgs.br.

## 1. COVID evolution in partition based on people pendular migration

The figures in this sections complement section 3.1 in the paper.

### 1.1. Clustering pendulum migration

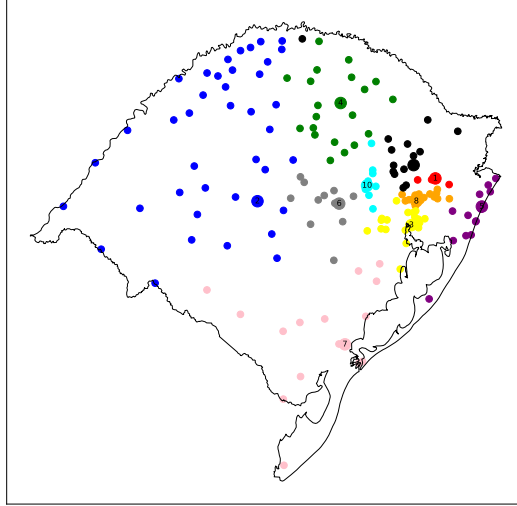

Figure 1: Same partition of Figure 1 in the paper, with clusters numbered in their largest cities.

## 1.2. Cluster 1

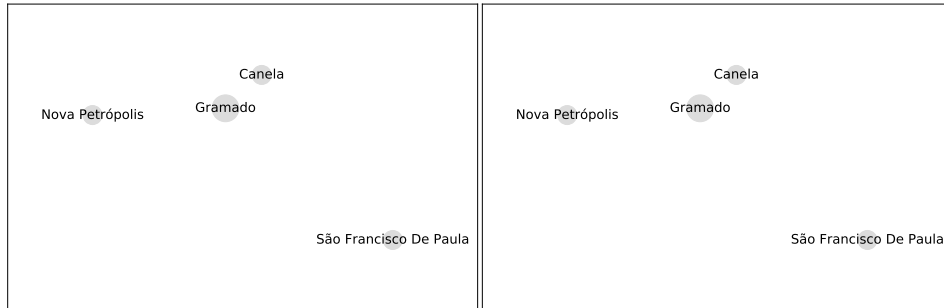

Figure 2: March 7-13 (left) and March 14-20 (right).

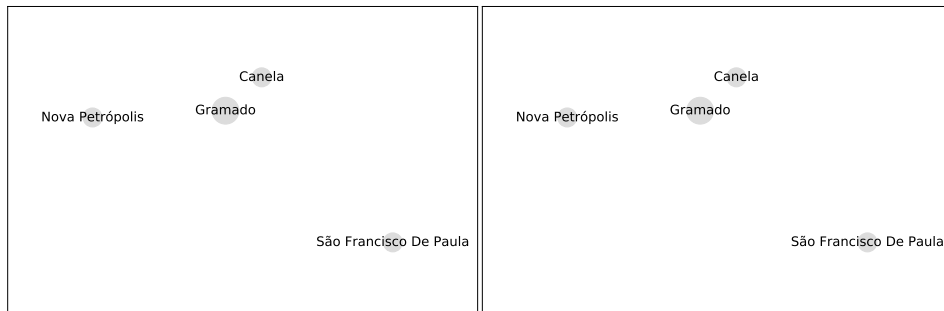

Figure 3: March 21-27 (left) and March 28 to April 3 (right).

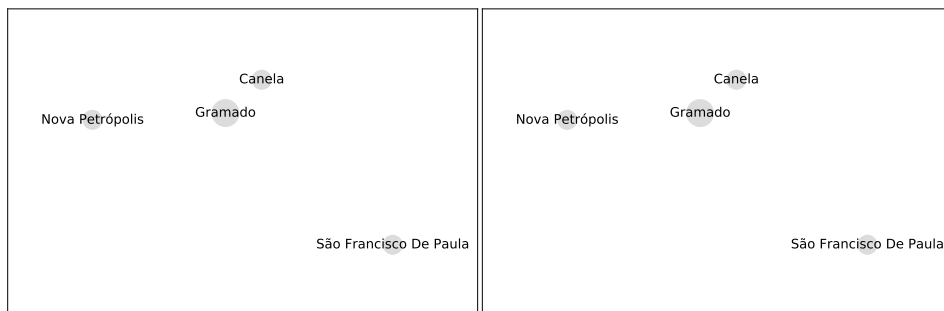

Figure 4: April 4-10 (left) and April 11-17 (right).

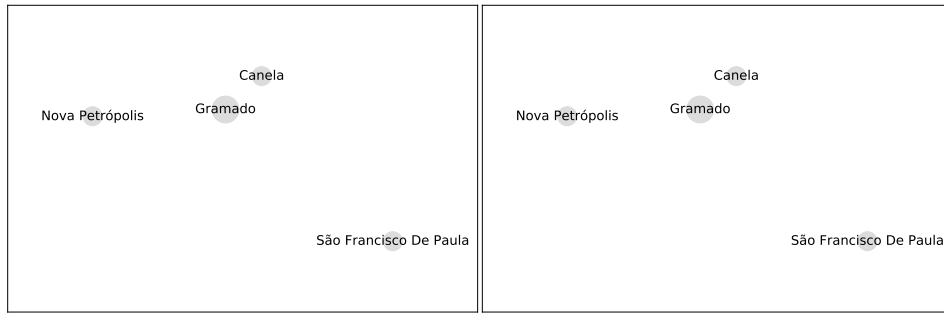

Figure 5: April 18-24 (left) and April 25 to May 1 (right).

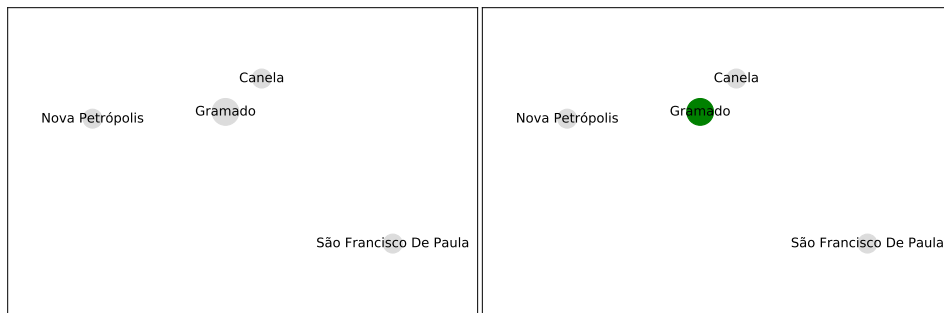

Figure 6: May 2-8 (left) and May 9-15 (right).

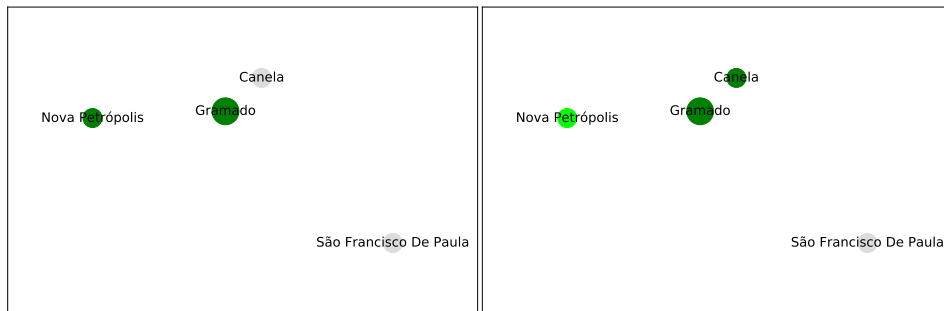

Figure 7: May 16-22 (left) and May 23-29 (right).

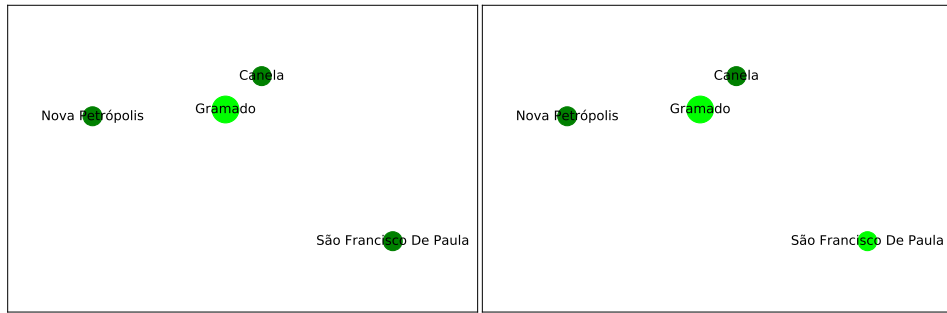

Figure 8: May 30 to June 5 (left) and June 6-12 (right).

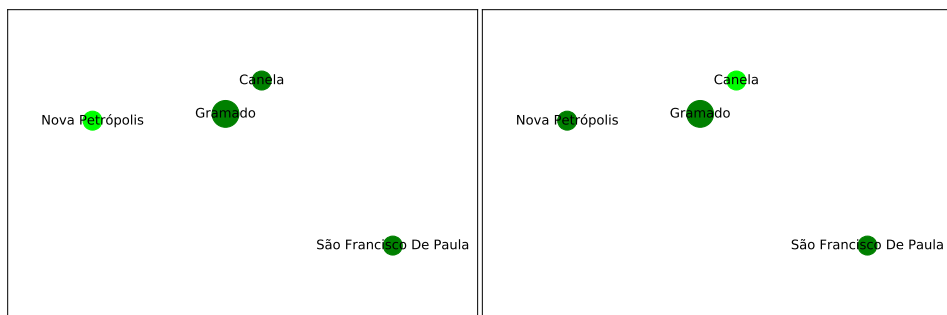

Figure 9: June 13-19 (left) and June 20-26 (right).

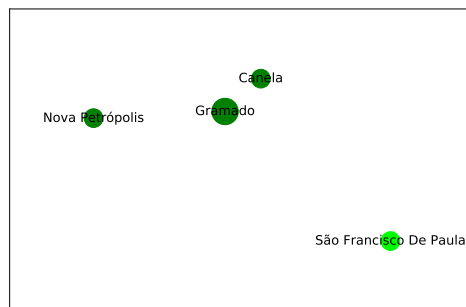

Figure 10: June 27 to July 3

### 1.3. Cluster 2

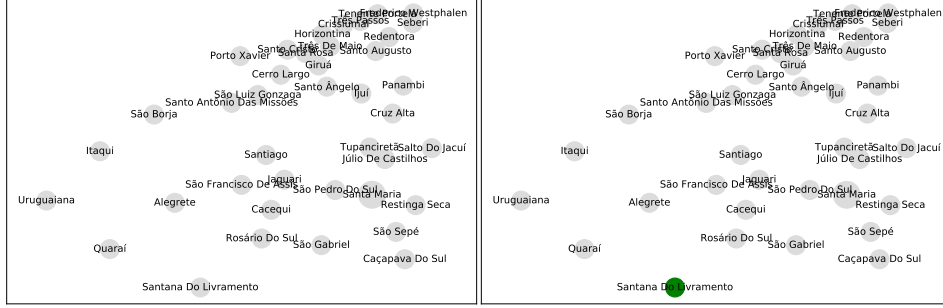

Figure 11: March 7-13 (left) and March 14-20 (right).

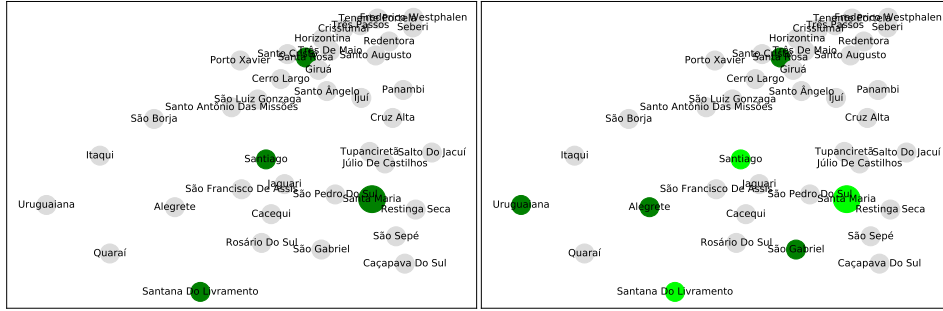

Figure 12: March 21-27 (left) and March 28 to April 3 (right).

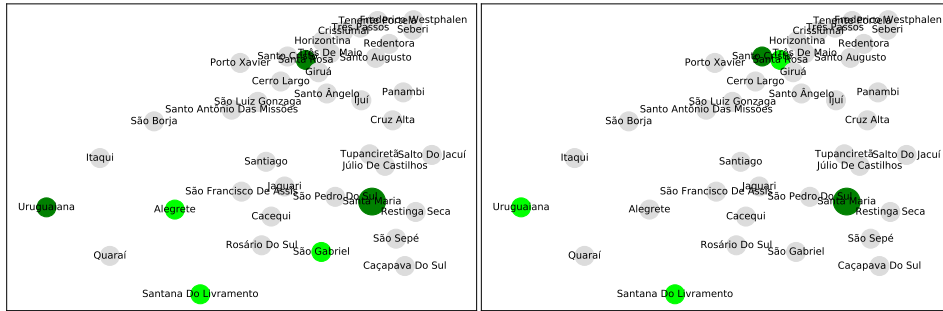

Figure 13: April 4-10 (left) and April 11-17 (right).

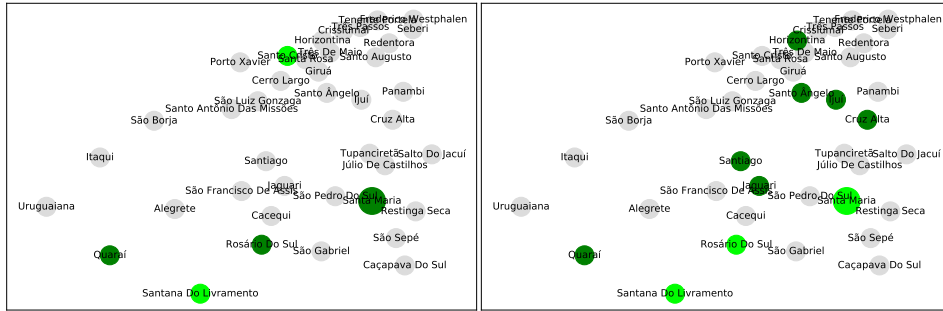

Figure 14: April 18-24 (left) and April 25 to May 1 (right).

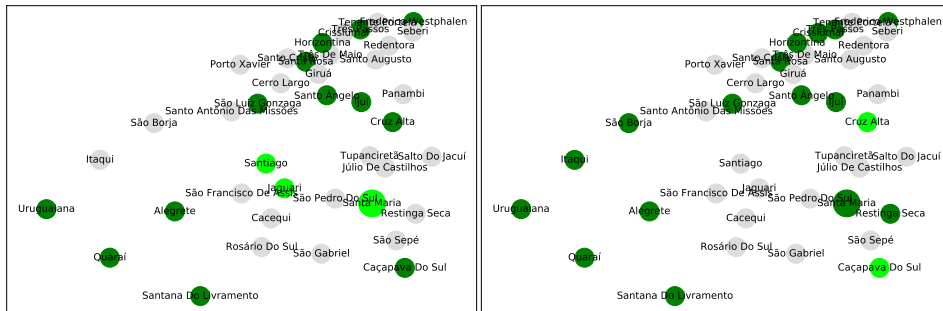

Figure 15: May 2-8 (left) and May 9-15 (right).

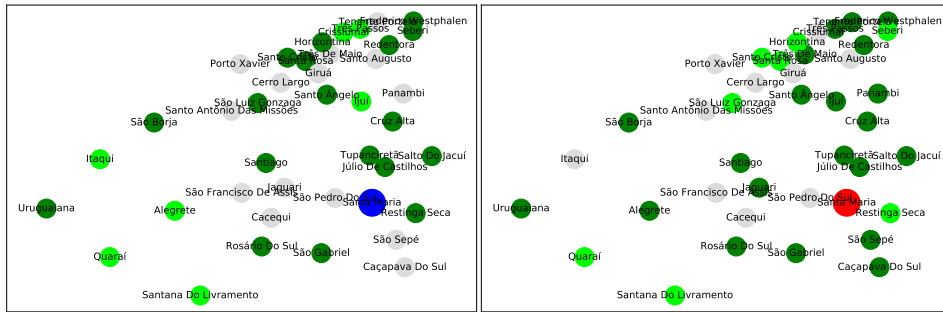

Figure 16: May 16-22 (left) and May 23-29 (right).

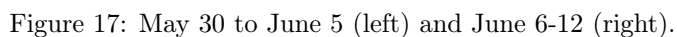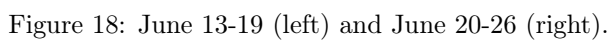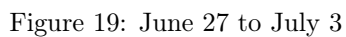

### 1.4. Cluster 3

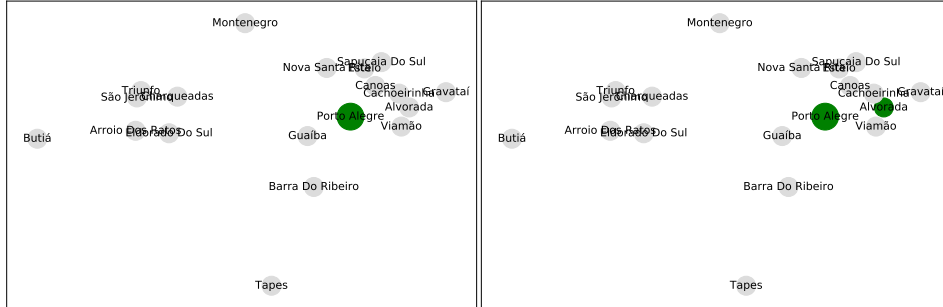

Figure 20: March 7-13 (left) and March 14-20 (right).

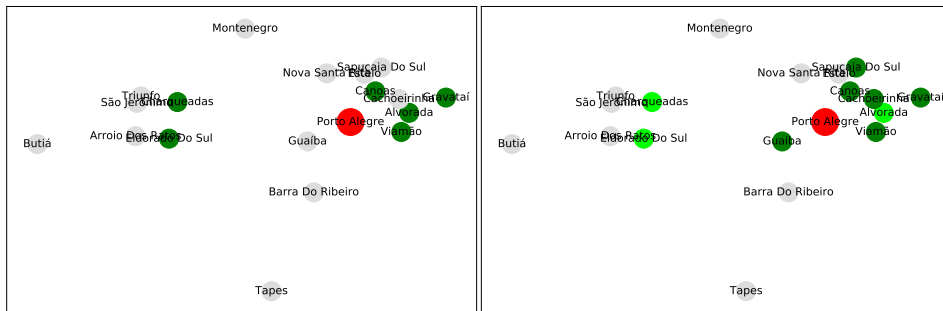

Figure 21: March 21-27 (left) and March 28 to April 3 (right).

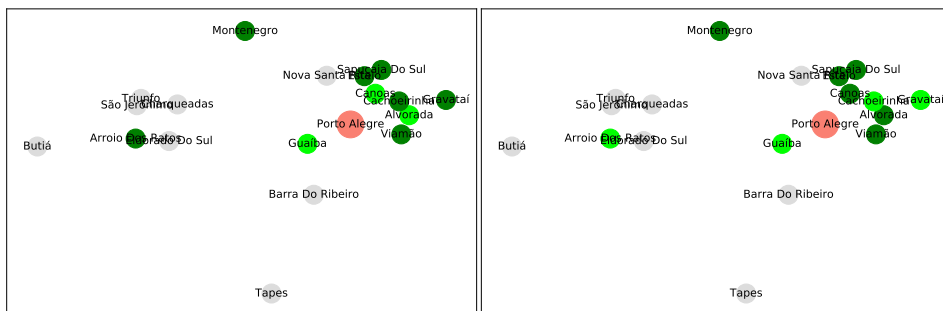

Figure 22: April 4-10 (left) and April 11-17 (right).

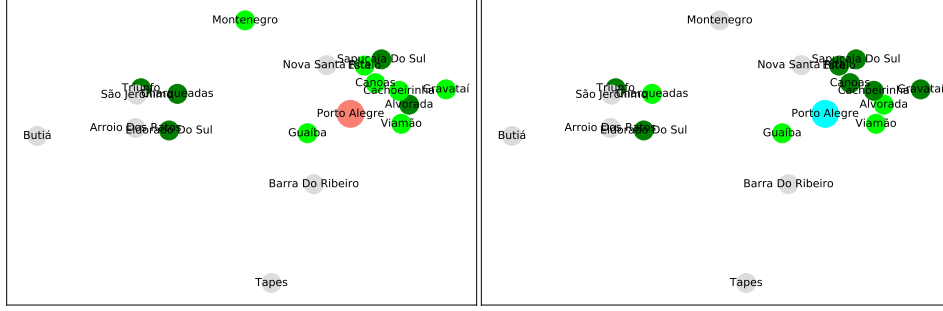

Figure 23: April 18-24 (left) and April 25 to May 1 (right).

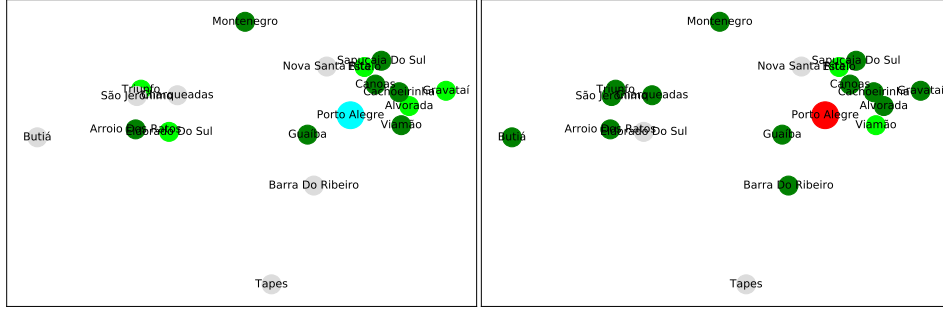

Figure 24: May 2-8 (left) and May 9-15 (right).

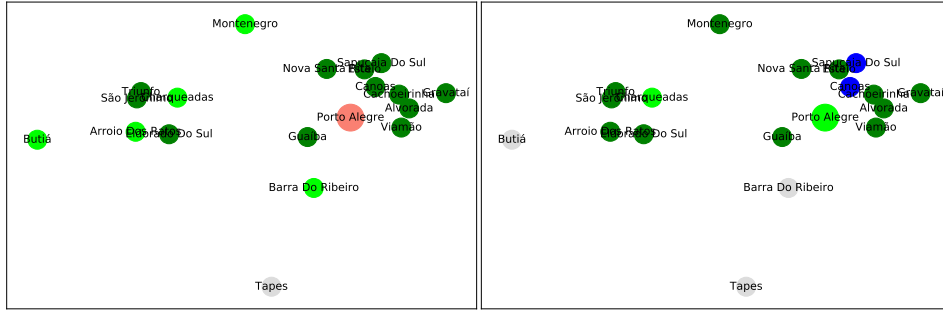

Figure 25: May 16-22 (left) and May 23-29 (right).

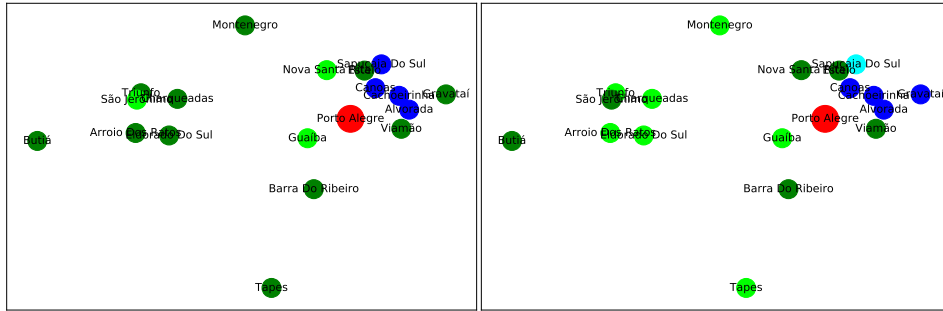

Figure 26: May 30 to June 5 (left) and June 6-12 (right).

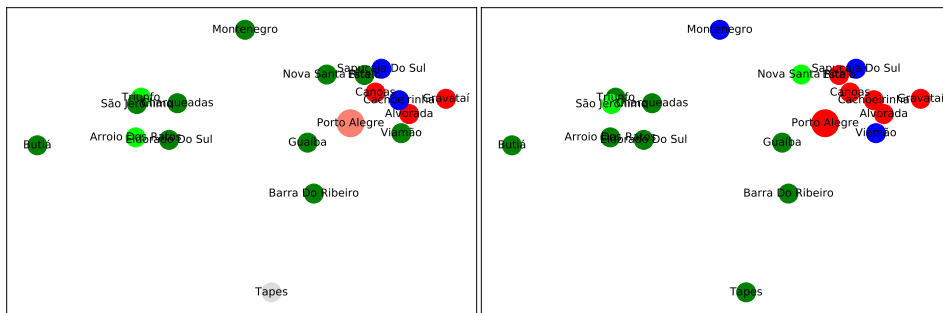

Figure 27: June 13-19 (left) and June 20-26 (right).

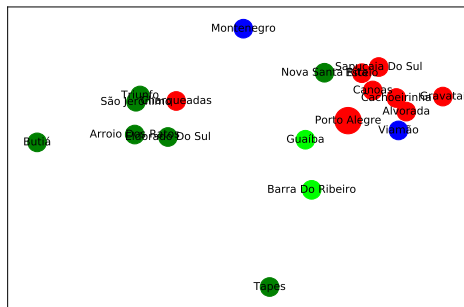

Figure 28: June 27 to July 3

### 1.5. Cluster 4

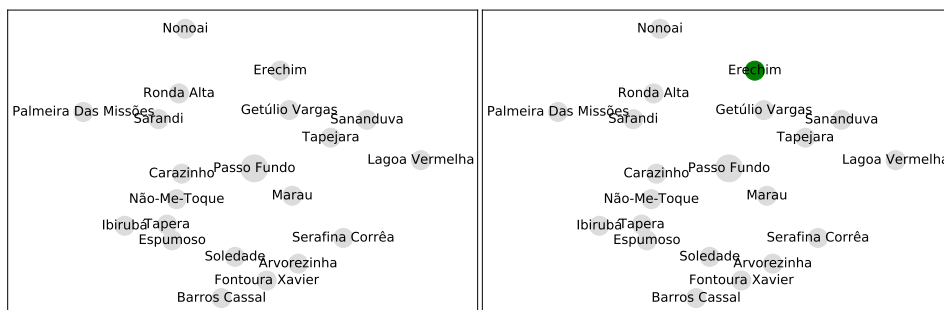

Figure 29: March 7-13 (left) and March 14-20 (right).

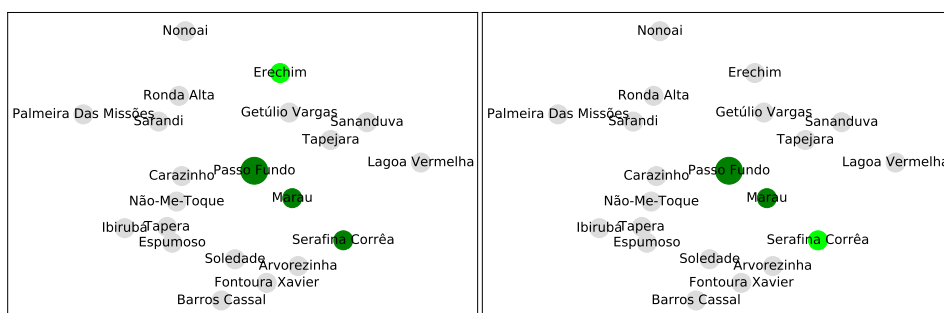

Figure 30: March 21-27 (left) and March 28 to April 3 (right).

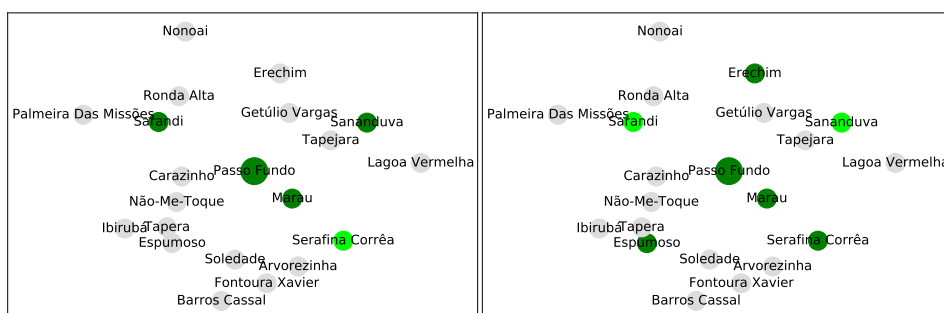

Figure 31: April 4-10 (left) and April 11-17 (right).

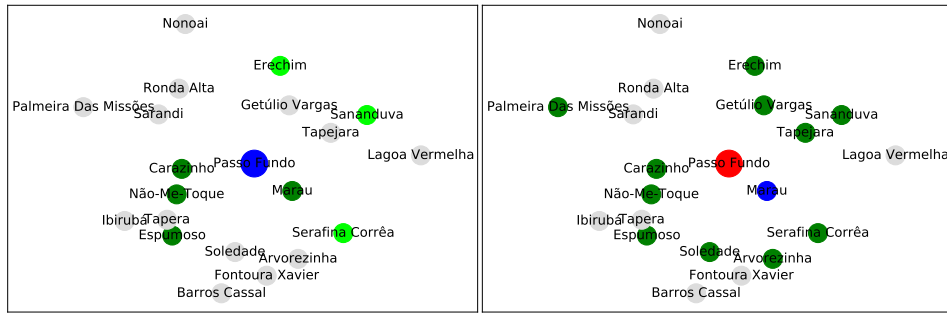

Figure 32: April 18-24 (left) and April 25 to May 1 (right).

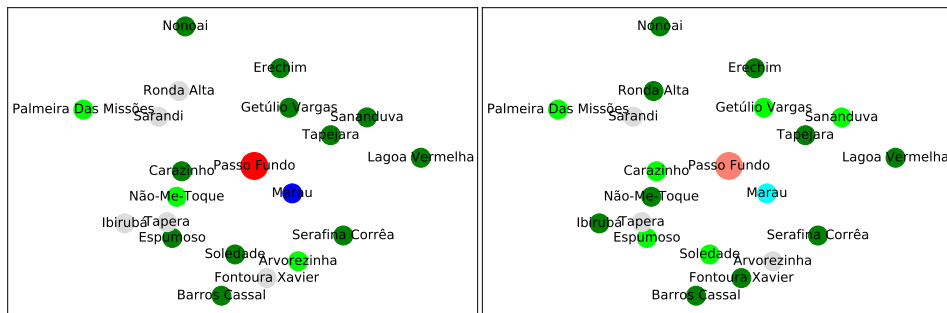

Figure 33: May 2-8 (left) and May 9-15 (right).

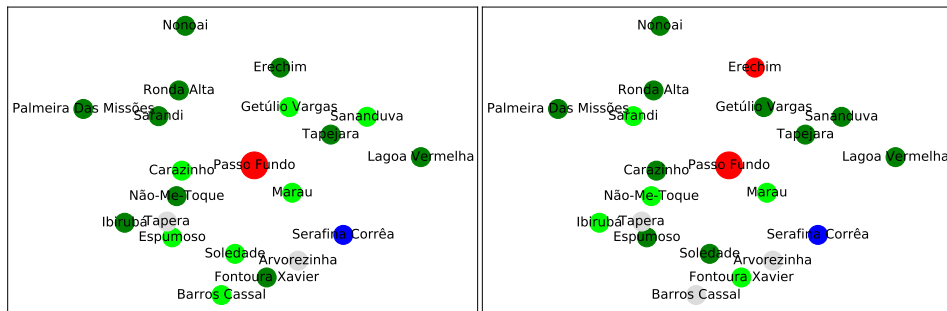

Figure 34: May 16-22 (left) and May 23-29 (right).

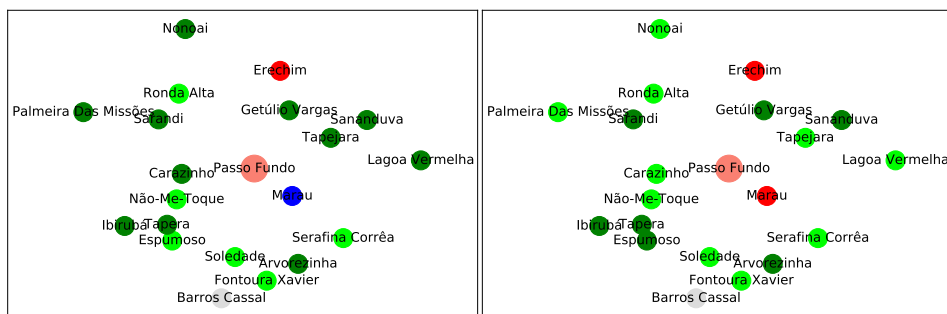

Figure 35: May 30 to June 5 (left) and June 6-12 (right).

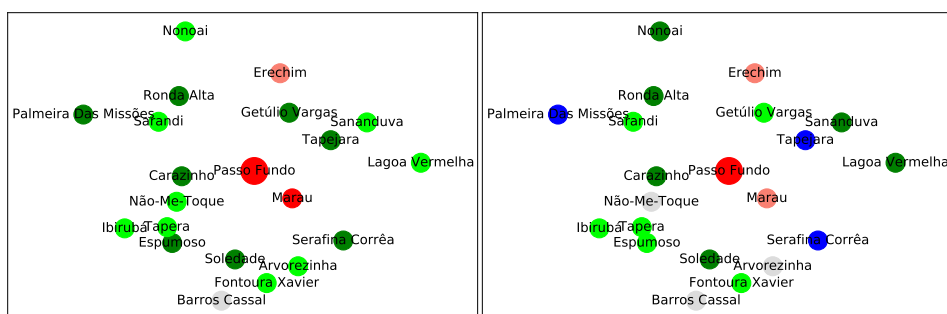

Figure 36: June 13-19 (left) and June 20-26 (right).

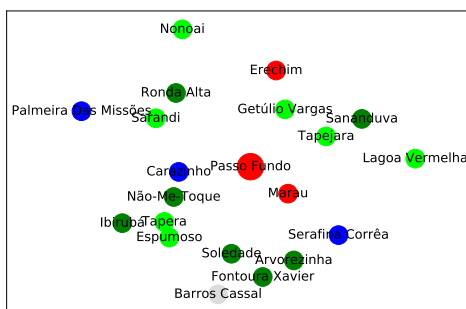

Figure 37: June 27 to July 3

## 1.6. Cluster 5

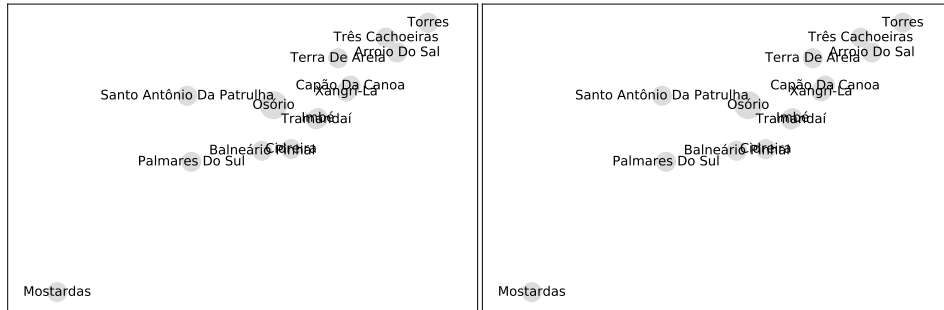

Figure 38: March 7-13 (left) and March 14-20 (right).

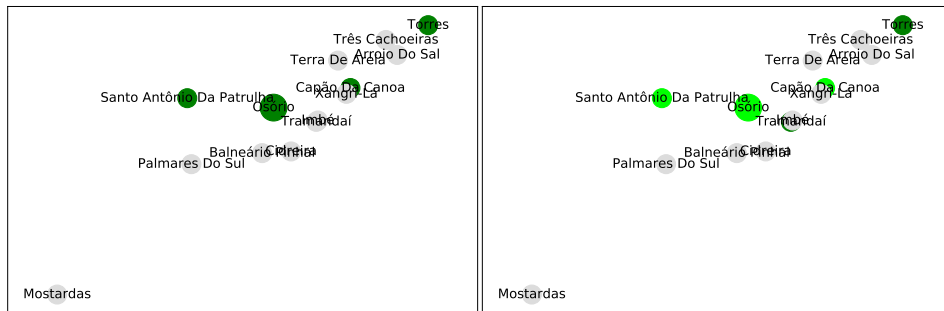

Figure 39: March 21-27 (left) and March 28 to April 3 (right).

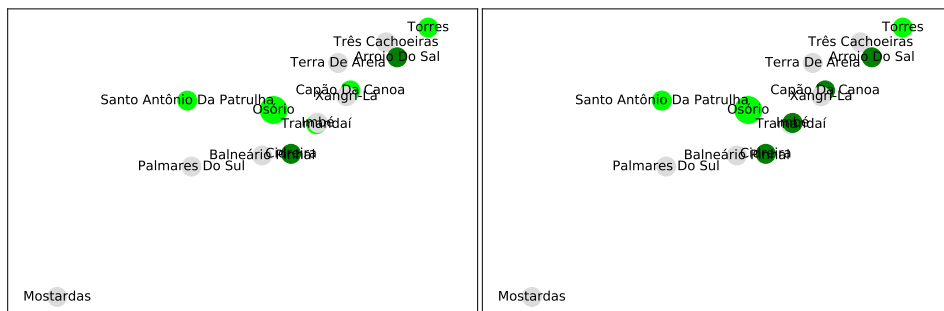

Figure 40: April 4-10 (left) and April 11-17 (right).

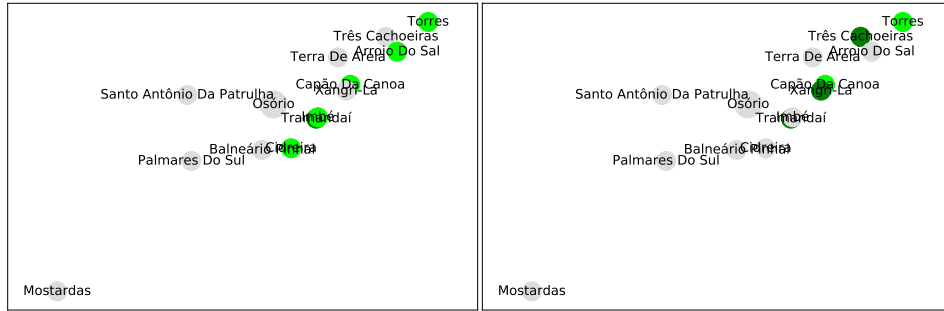

Figure 41: April 18-24 (left) and April 25 to May 1 (right).

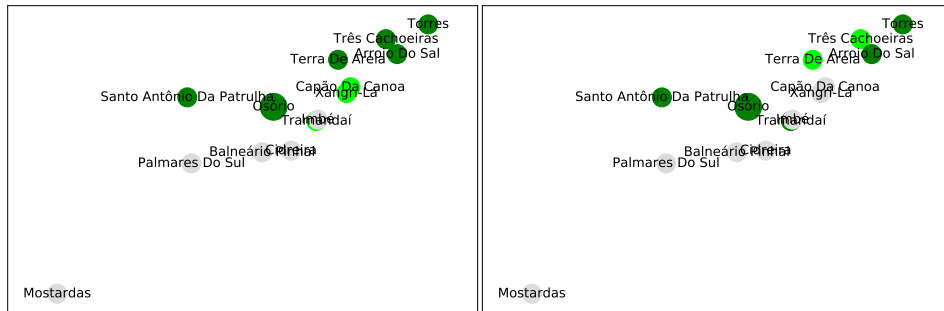

Figure 42: May 2-8 (left) and May 9-15 (right).

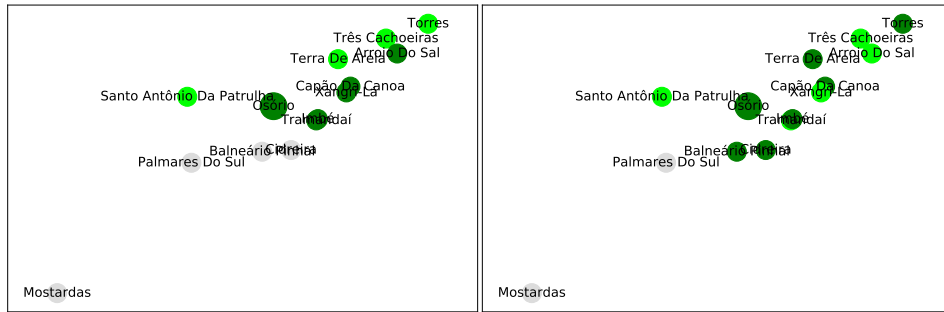

Figure 43: May 16-22 (left) and May 23-29 (right).

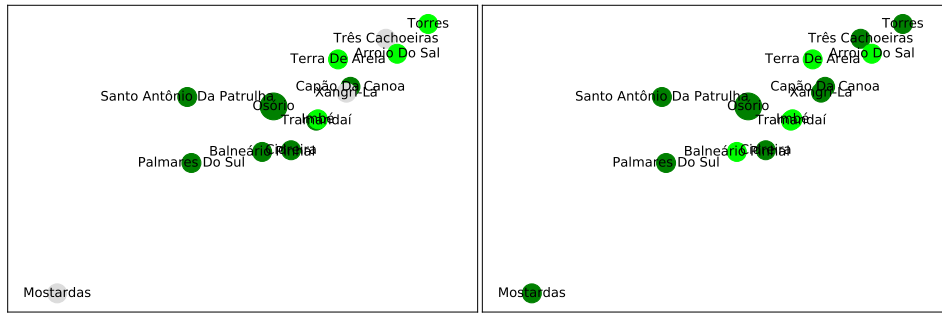

Figure 44: May 30 to June 5 (left) and June 6-12 (right).

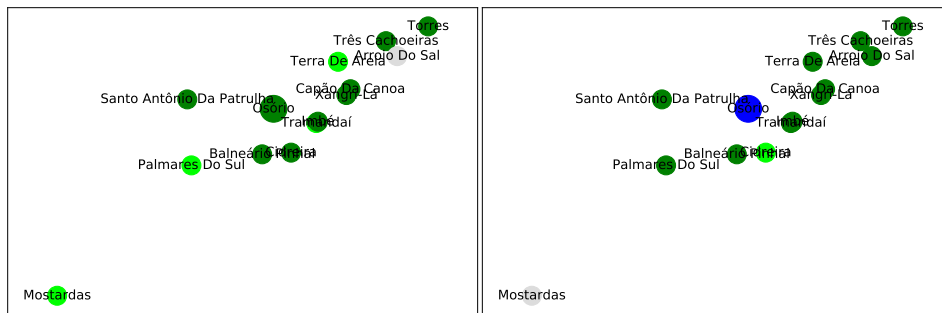

Figure 45: June 13-19 (left) and June 20-26 (right).

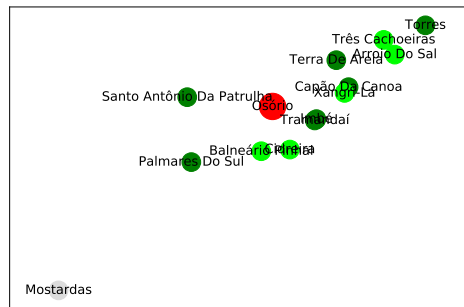

Figure 46: June 27 to July 3

**1.7. Cluster 6**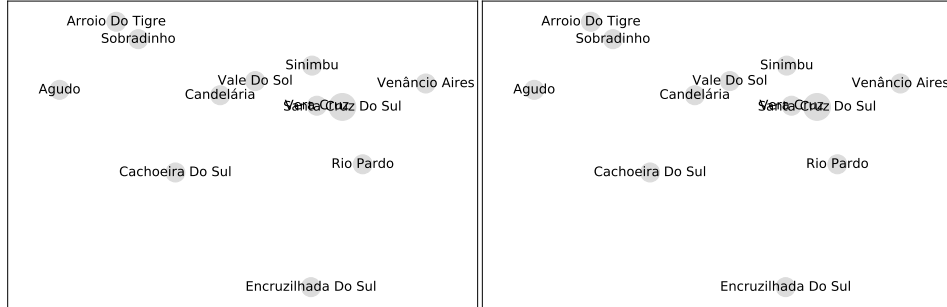

Figure 47: March 7-13 (left) and March 14-20 (right).

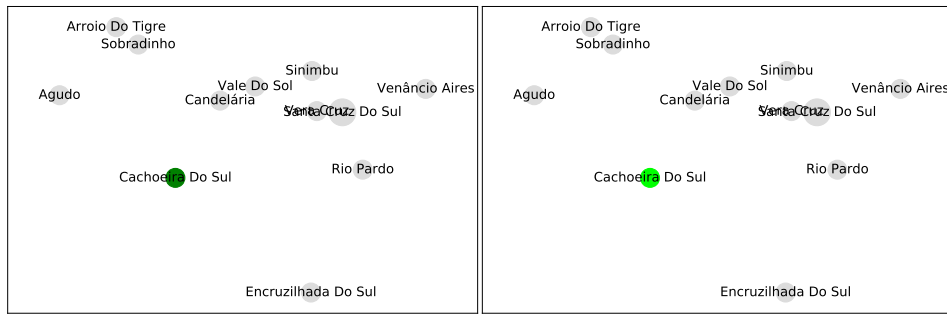

Figure 48: March 21-27 (left) and March 28 to April 3 (right).

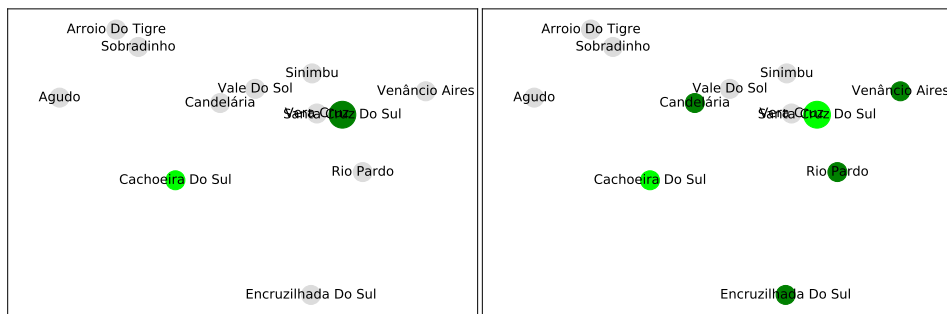

Figure 49: April 4-10 (left) and April 11-17 (right).

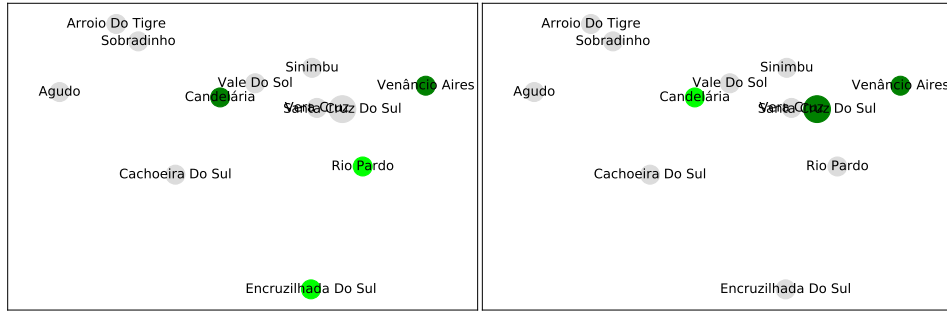

Figure 50: April 18-24 (left) and April 25 to May 1 (right).

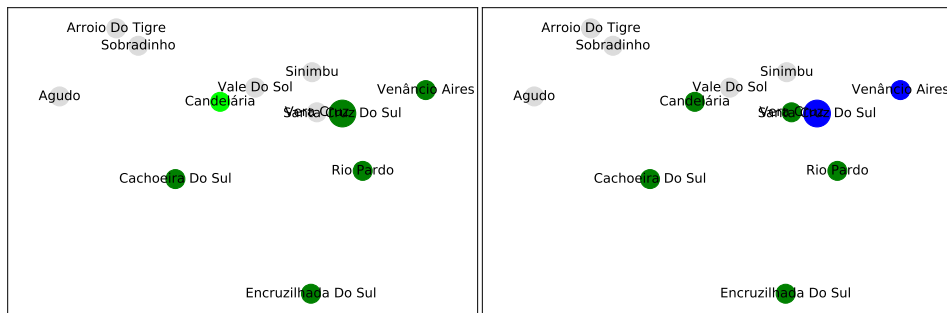

Figure 51: May 2-8 (left) and May 9-15 (right).

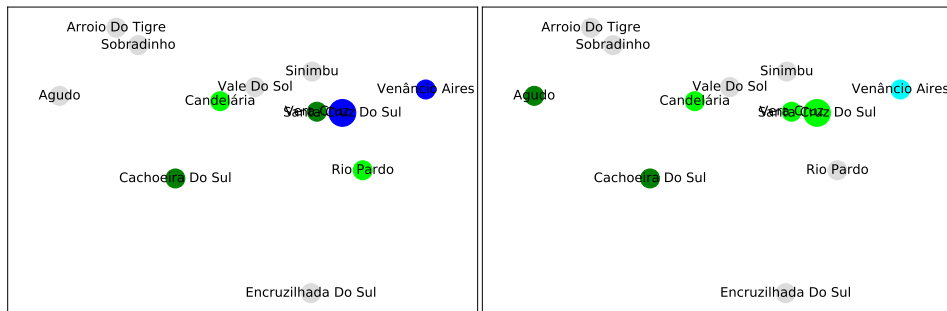

Figure 52: May 16-22 (left) and May 23-29 (right).

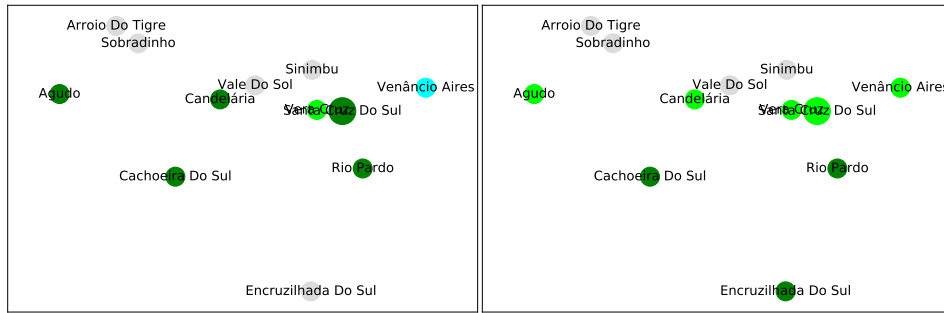

Figure 53: May 30 to June 5 (left) and June 6-12 (right).

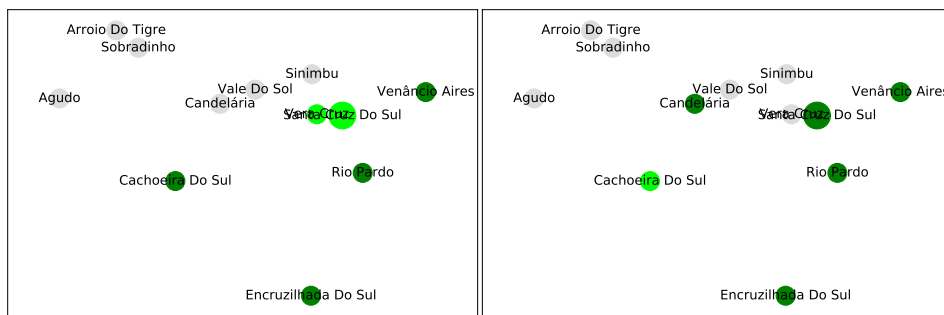

Figure 54: June 13-19 (left) and June 20-26 (right).

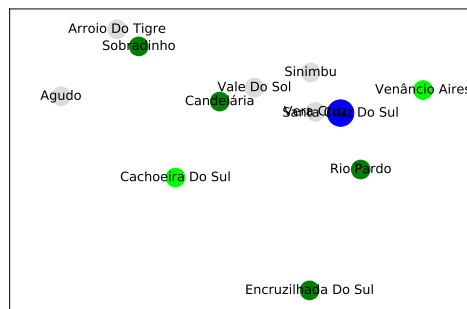

Figure 55: June 27 to July 3

## 1.8. Cluster 7

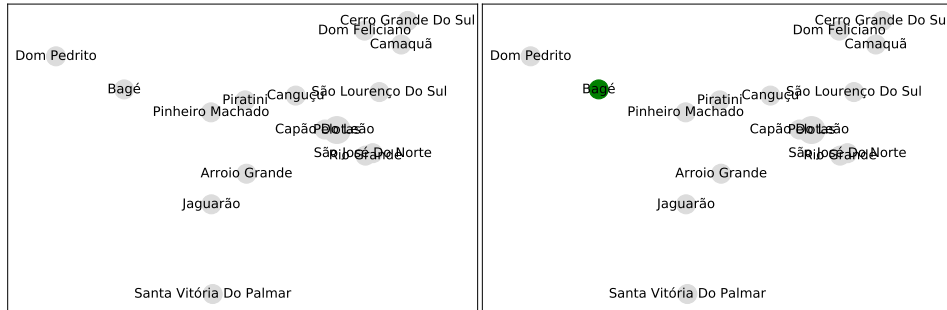

Figure 56: March 7-13 (left) and March 14-20 (right).

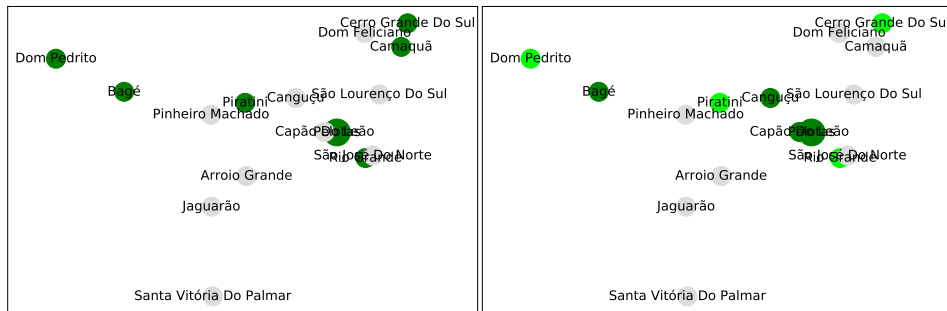

Figure 57: March 21-27 (left) and March 28 to April 3 (right).

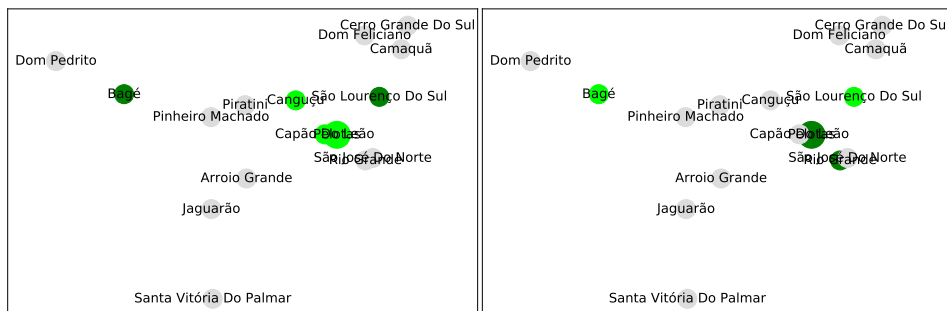

Figure 58: April 4-10 (left) and April 11-17 (right).

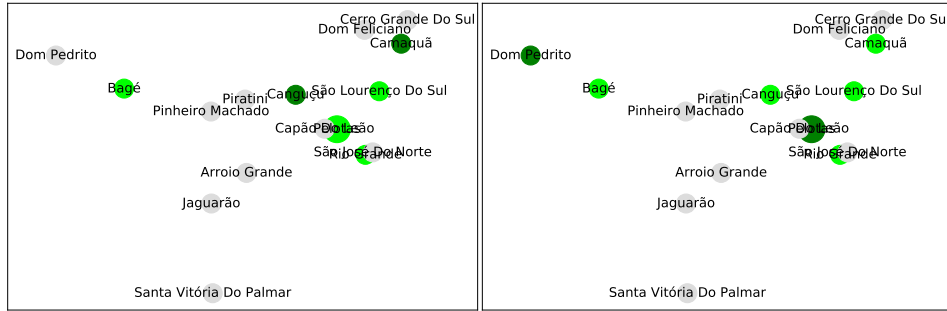

Figure 59: April 18-24 (left) and April 25 to May 1 (right).

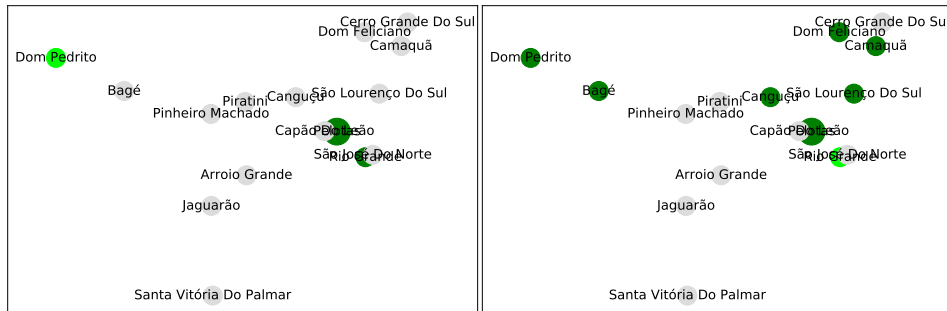

Figure 60: May 2-8 (left) and May 9-15 (right).

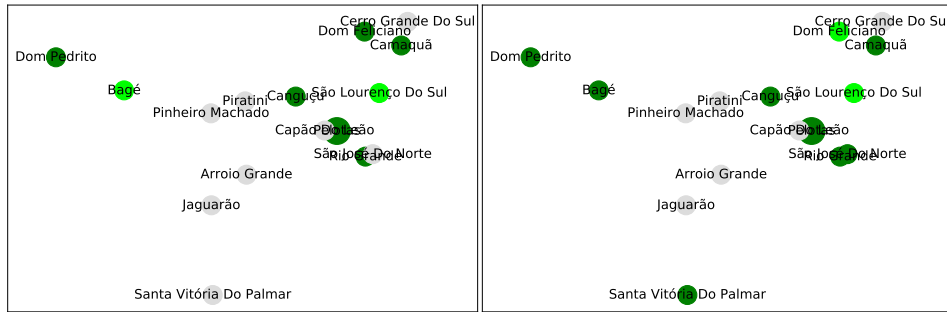

Figure 61: May 16-22 (left) and May 23-29 (right).

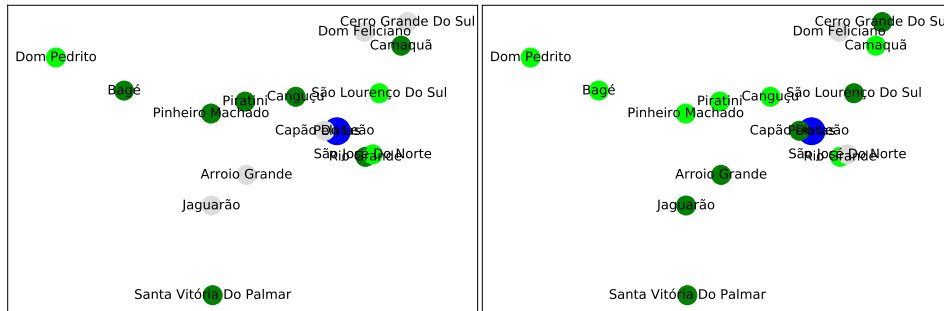

Figure 62: May 30 to June 5 (left) and June 6-12 (right).

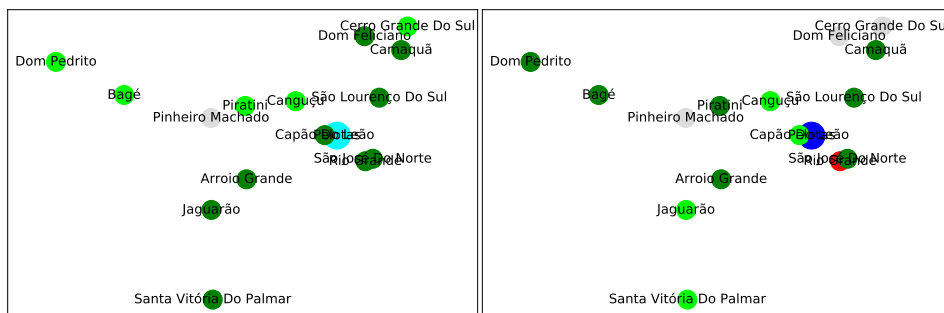

Figure 63: June 13-19 (left) and June 20-26 (right).

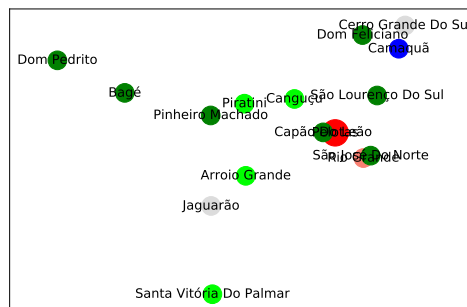

Figure 64: June 27 to July 3

### 1.9. Cluster 8

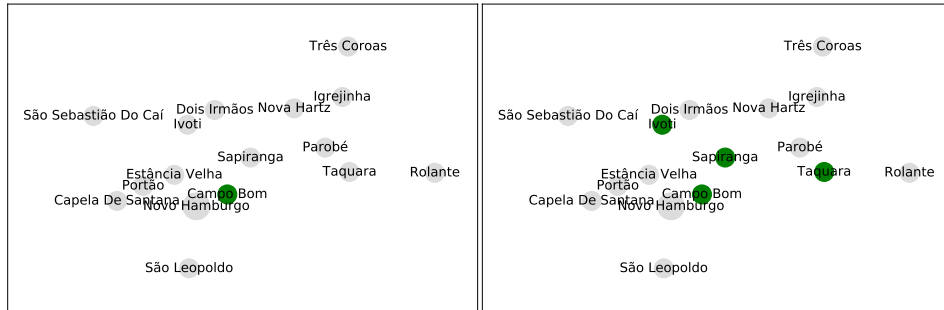

Figure 65: March 7-13 (left) and March 14-20 (right).

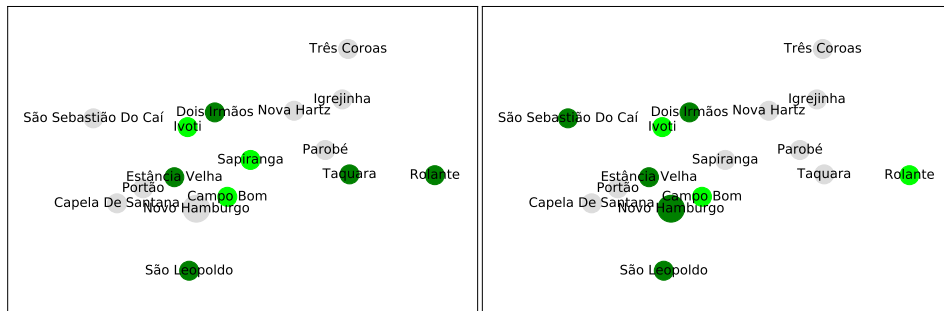

Figure 66: March 21-27 (left) and March 28 to April 3 (right).

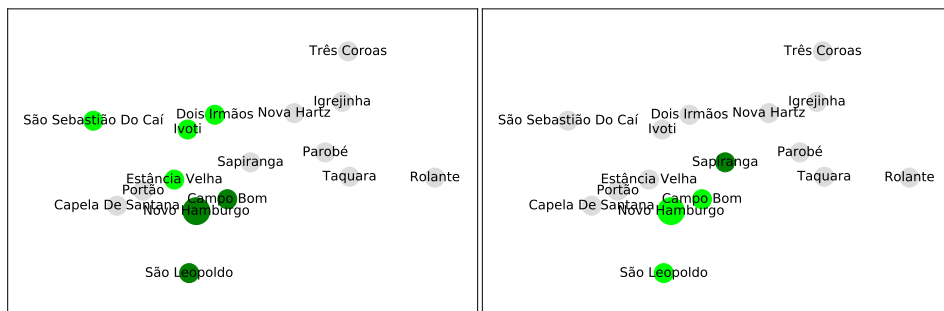

Figure 67: April 4-10 (left) and April 11-17 (right).

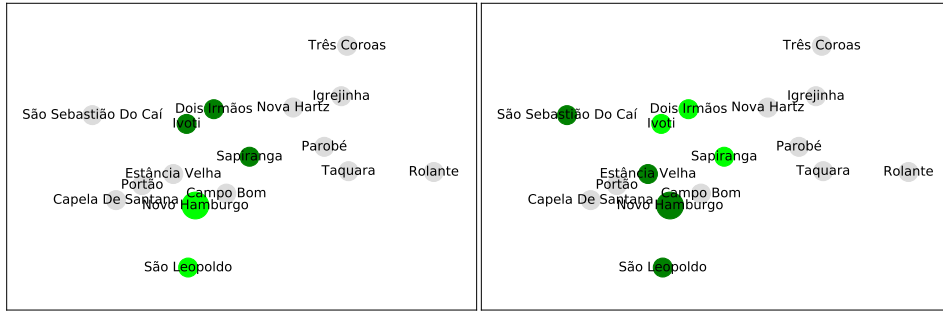

Figure 68: April 18-24 (left) and April 25 to May 1 (right).

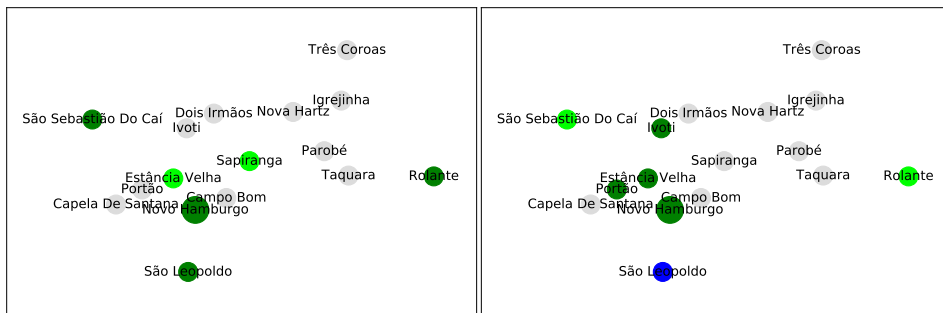

Figure 69: May 2-8 (left) and May 9-15 (right).

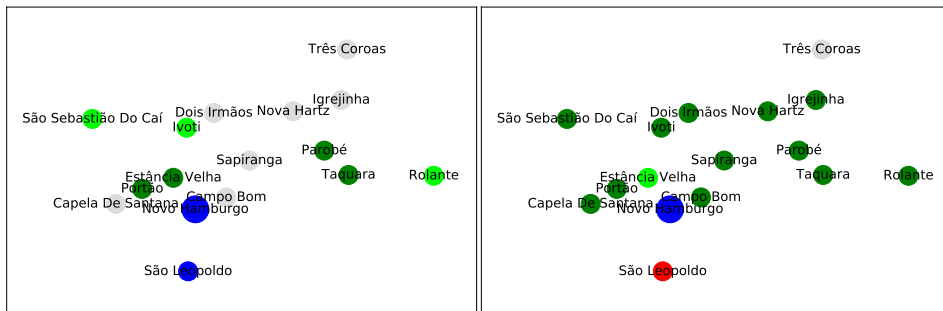

Figure 70: May 16-22 (left) and May 23-29 (right).

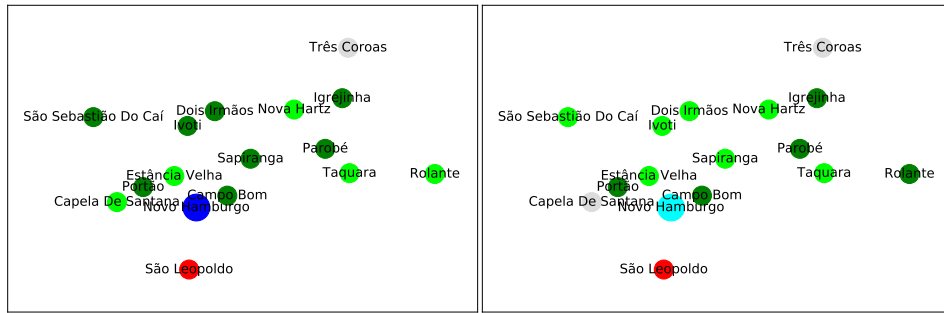

Figure 71: May 30 to June 5 (left) and June 6-12 (right).

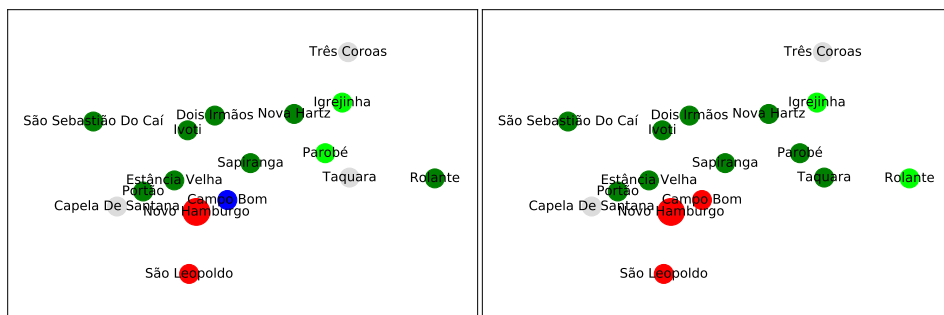

Figure 72: June 13-19 (left) and June 20-26 (right).

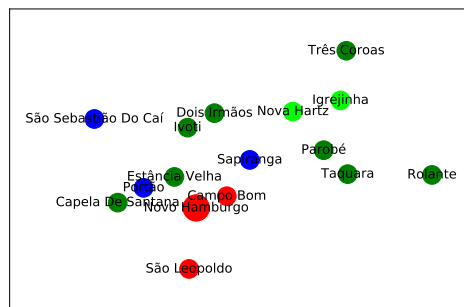

Figure 73: June 27 to July 3

### 1.10. Cluster 9

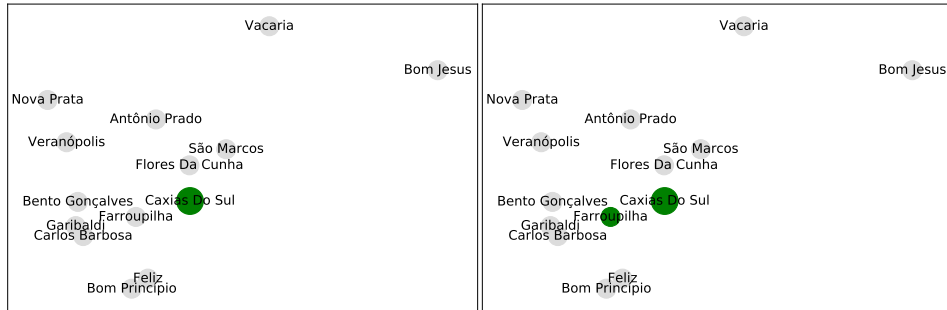

Figure 74: March 7-13 (left) and March 14-20 (right).

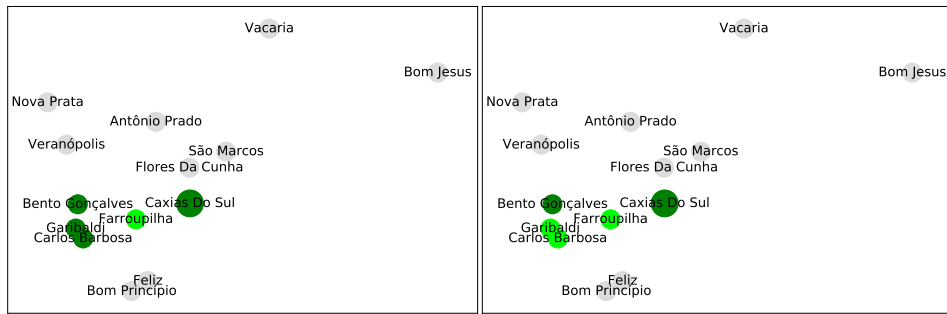

Figure 75: March 21-27 (left) and March 28 to April 3 (right).

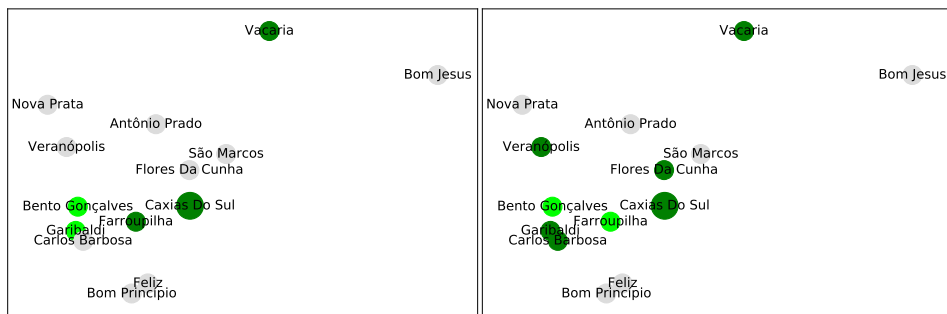

Figure 76: April 4-10 (left) and April 11-17 (right).

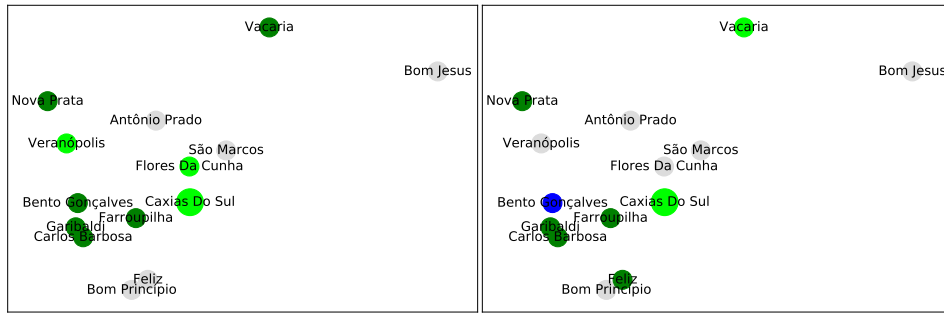

Figure 77: April 18-24 (left) and April 25 to May 1 (right).

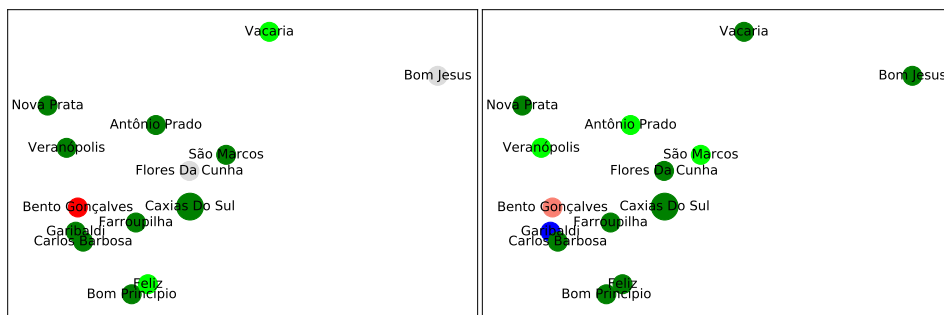

Figure 78: May 2-8 (left) and May 9-15 (right).

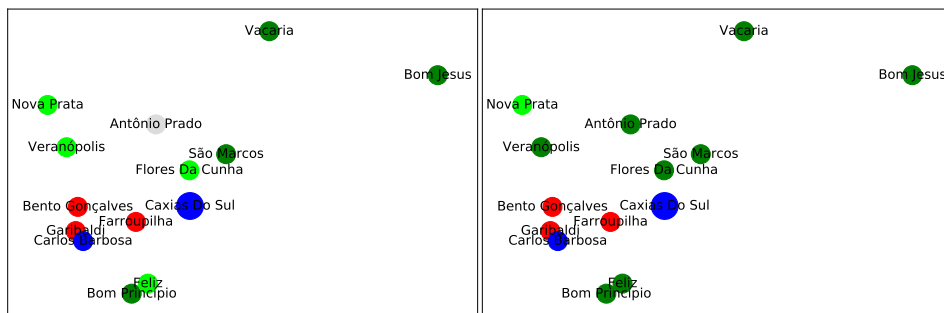

Figure 79: May 16-22 (left) and May 23-29 (right).

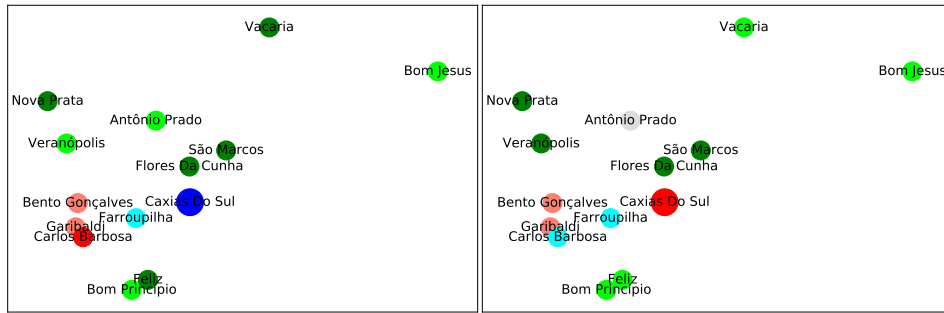

Figure 80: May 30 to June 5 (left) and June 6-12 (right).

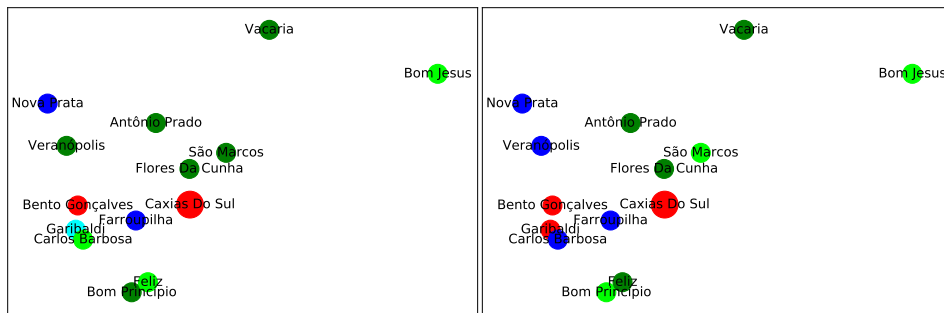

Figure 81: June 13-19 (left) and June 20-26 (right).

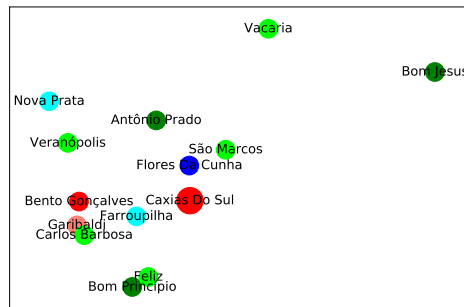

Figure 82: June 27 to July 3

**1.11. Cluster 10**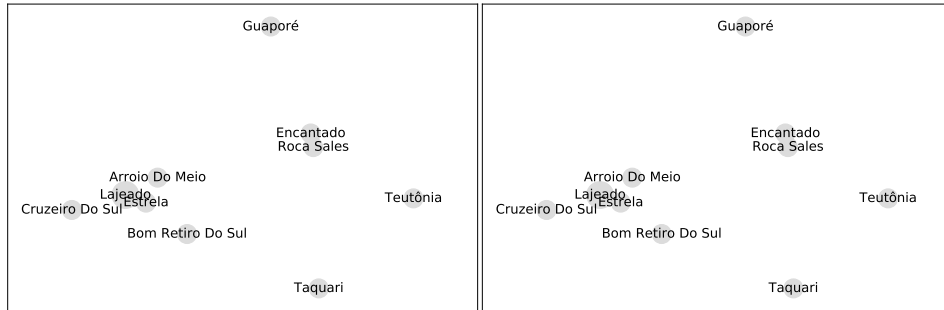

Figure 83: March 7-13 (left) and March 14-20 (right).

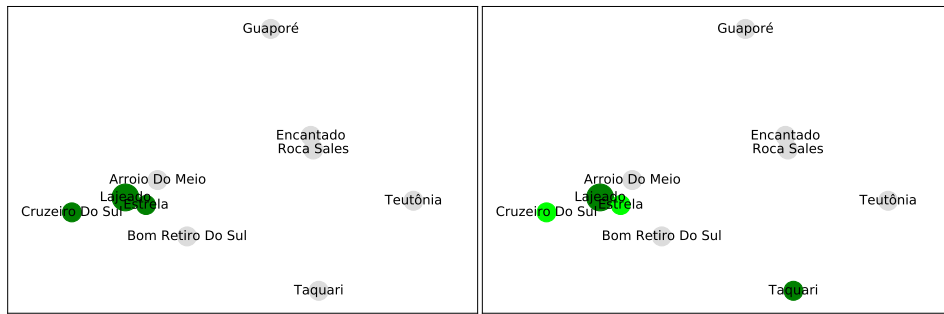

Figure 84: March 21-27 (left) and March 28 to April 3 (right).

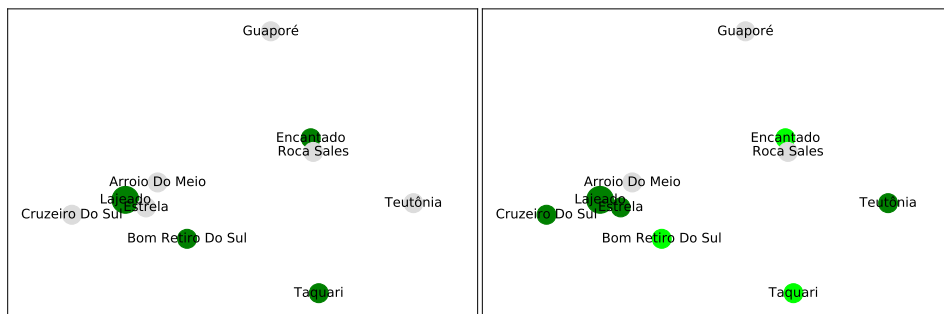

Figure 85: April 4-10 (left) and April 11-17 (right).

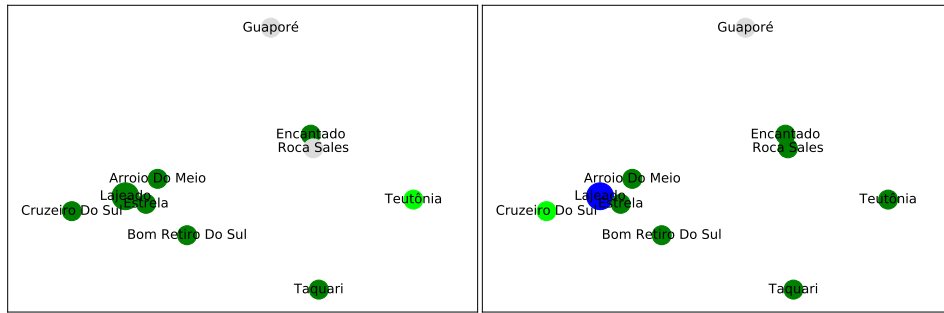

Figure 86: April 18-24 (left) and April 25 to May 1 (right).

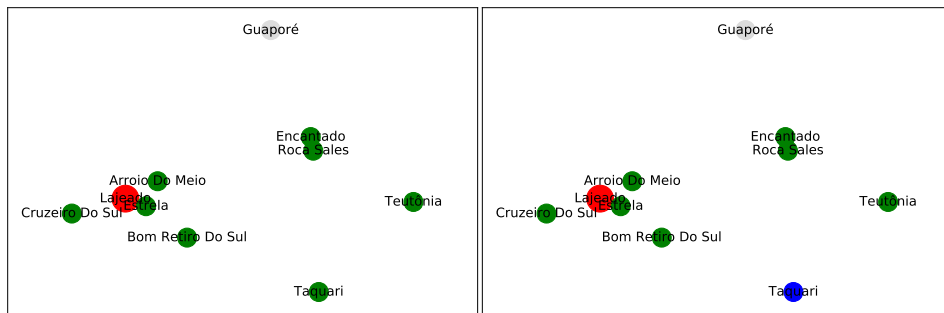

Figure 87: May 2-8 (left) and May 9-15 (right).

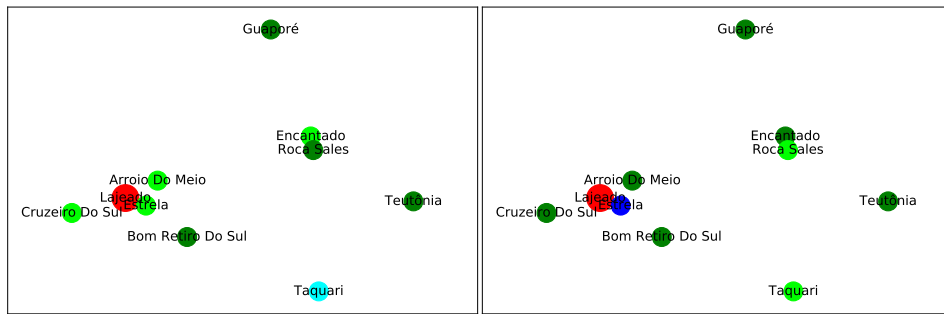

Figure 88: May 16-22 (left) and May 23-29 (right).

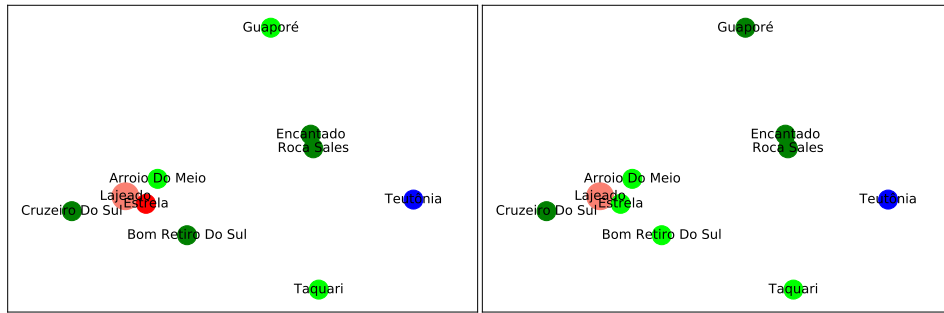

Figure 89: May 30 to June 5 (left) and June 6-12 (right).

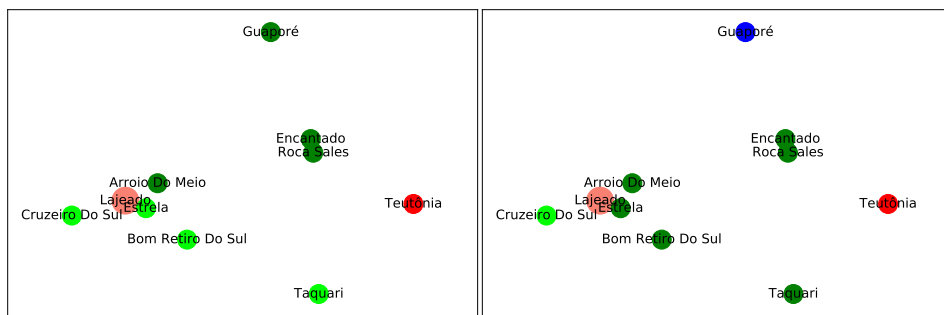

Figure 90: June 13-19 (left) and June 20-26 (right).

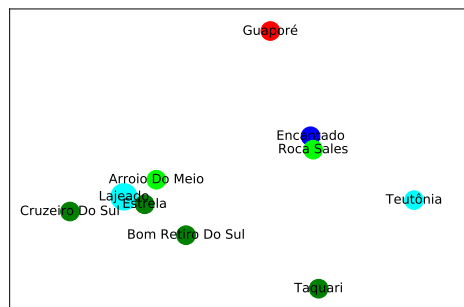

Figure 91: June 27 to July 3

## 2. Clustering based on available ICU beds

The figures in this sections complement section 3.2 in the paper.

### 2.1. Static partition based on total ICU beds

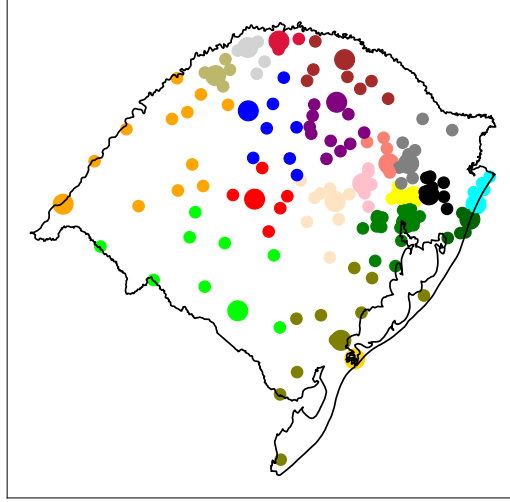

Figure 92: Partition obtained using total ICU beds in cities data, whose gap is  $\text{NCut}(\mathcal{P})/\text{ncut}_k^{rel}(G) \approx 1.0339$ .

## 2.2. Weekly partitions based on available ICU beds

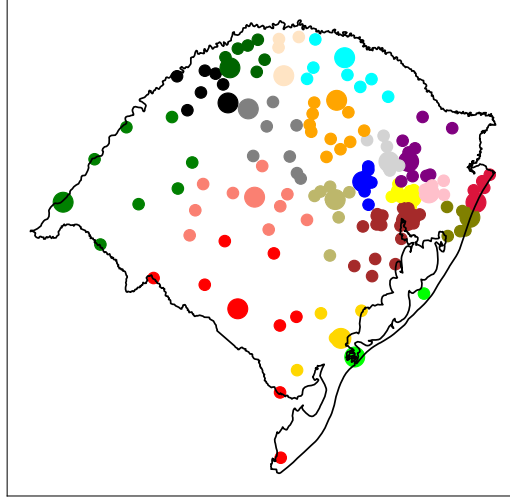

Figure 93: Partition obtained using data from week May 9-15, whose gap is  $\text{NCut}(\mathcal{P})/\text{ncut}_k^{rel}(G) \approx 1.0360$ .

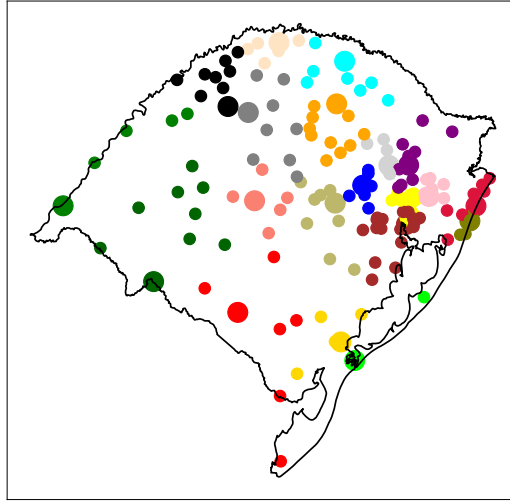

Figure 94: Partition obtained using data from week May 16-22, whose gap is  $\text{NCut}(\mathcal{P})/\text{ncut}_k^{rel}(G) \approx 1.0337$ .

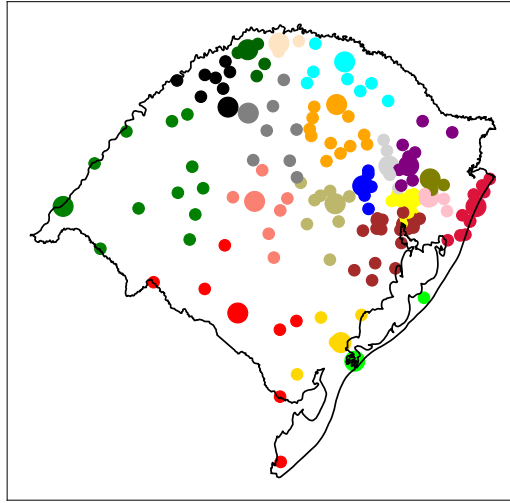

Figure 95: Partition obtained using data from week May 23-29, whose gap is  $\text{NCut}(\mathcal{P})/\text{ncut}_k^{\text{rel}}(G) \approx 1.0330$ .

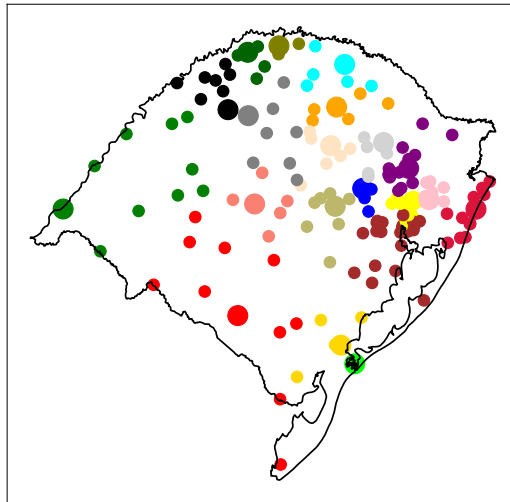

Figure 96: Partition obtained using data from week May 30 to June 5, whose gap is  $\text{NCut}(\mathcal{P})/\text{ncut}_k^{\text{rel}}(G) \approx 1.0330$ .

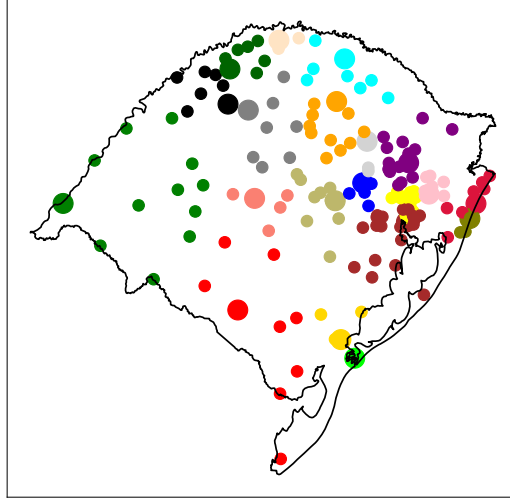

Figure 97: Partition obtained using data from week June 6-12, whose gap is  $\text{NCut}(\mathcal{P})/\text{ncut}_k^{\text{rel}}(G) \approx 1.0311$ .

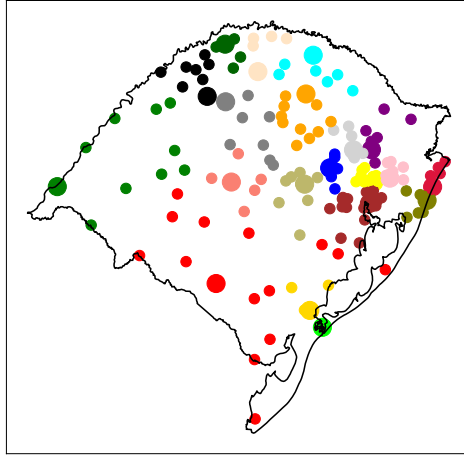

Figure 98: Partition obtained using data from week June 13-19, whose gap is  $\text{NCut}(\mathcal{P})/\text{ncut}_k^{\text{rel}}(G) \approx 1.0329$ .

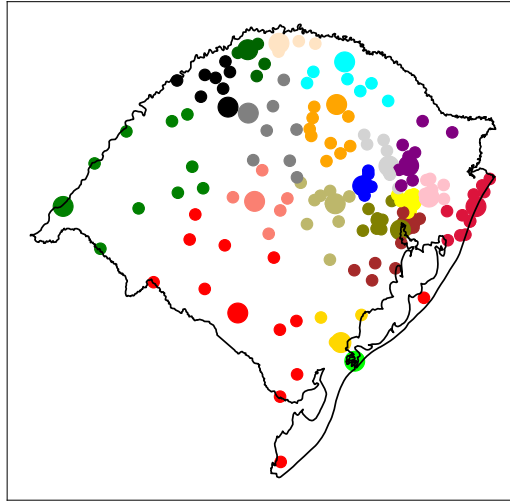

Figure 99: Partition obtained using data from week June 20-26, whose gap is  $\text{NCut}(\mathcal{P})/\text{ncut}_k^{\text{rel}}(G) \approx 1.0354$ .

### 2.3. Comparison of state's flags with our flags in state's regions

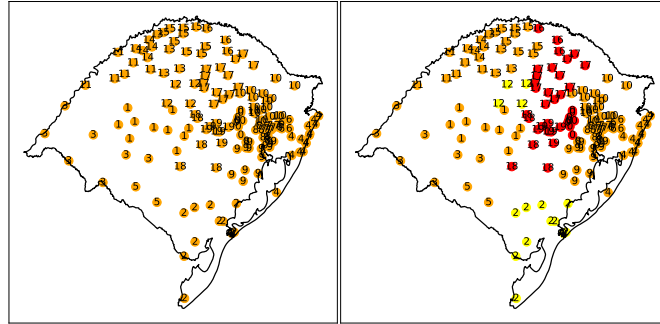

Figure 100: Flags assigned by the state formula (left) and by our formula (right) on the week May 9-15.

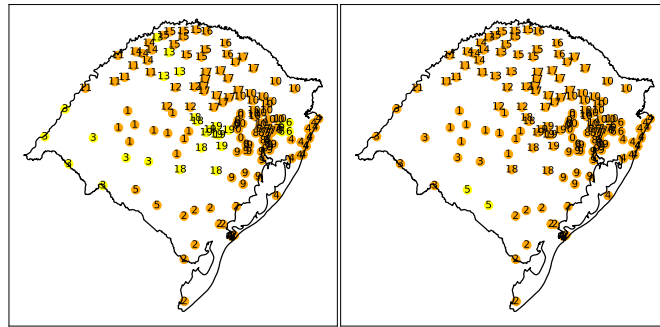

Figure 101: Flags assigned by the state formula (left) and by our formula (right) on the week May 16-22.

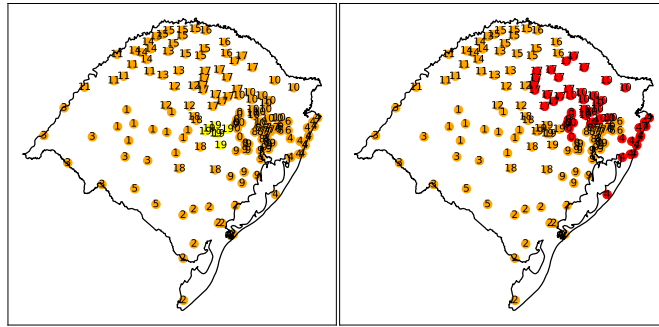

Figure 102: Flags assigned by the state formula (left) and by our formula (right) on the week May 23-29.

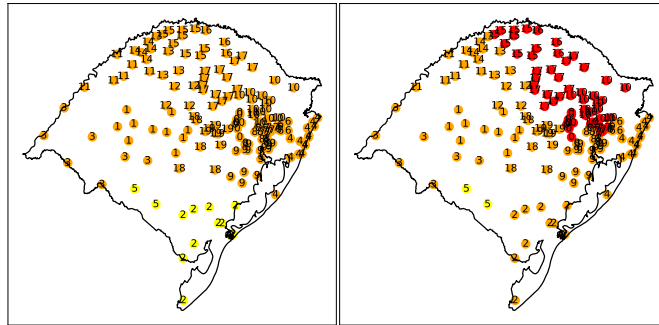

Figure 103: Flags assigned by the state formula (left) and by our formula (right) on the week May 30 to June 5.

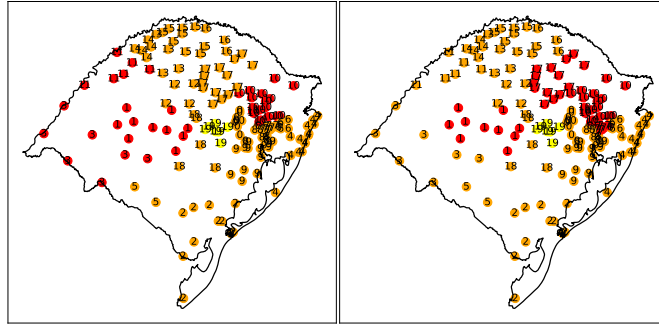

Figure 104: Flags assigned by the state formula (left) and by our formula (right) on the week June 6-12.

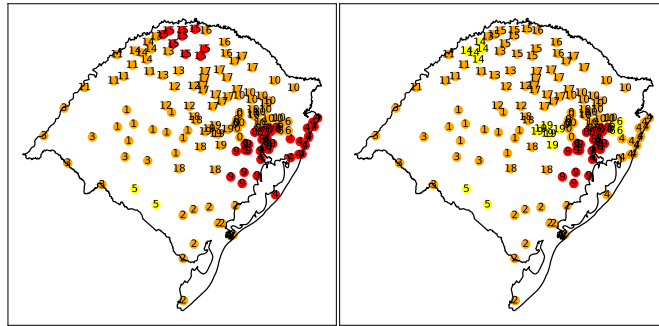

Figure 105: Flags assigned by the state formula (left) and by our formula (right) on the week June 13-19.

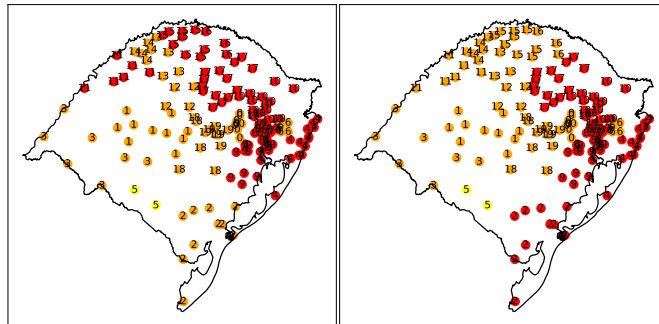

Figure 106: Flags assigned by the state formula (left) and by our formula (right) on the week June 20-26.

## 2.4. Our flags assigned to state's regions and to dynamic regions along seven weeks

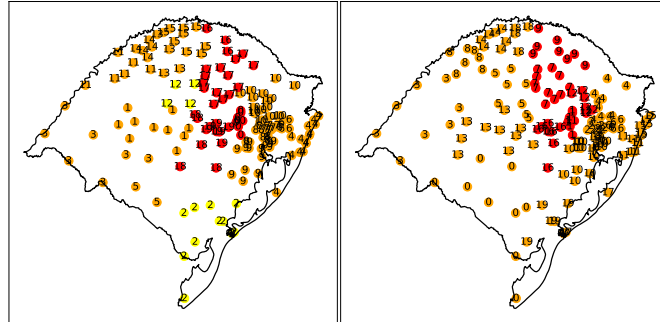

Figure 107: Flags assigned by our formula to the state's regions (left) and to the dynamic regions (right) on the week May 9-15.

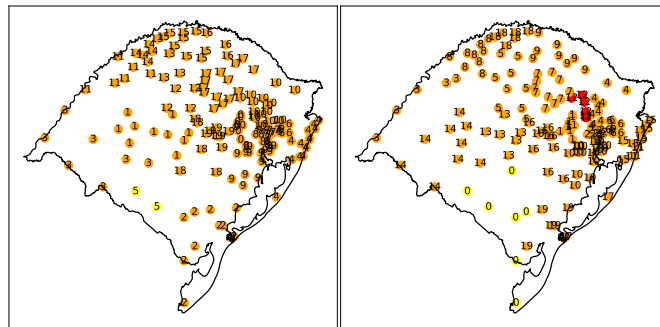

Figure 108: Flags assigned by our formula to the state's regions (left) and to the dynamic regions (right) on the week May 16-22.

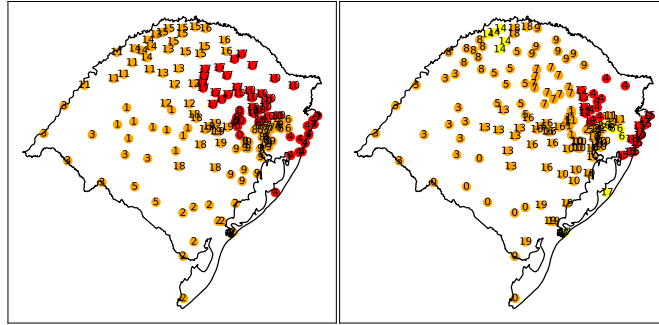

Figure 109: Flags assigned by our formula to the state's regions (left) and to the dynamic regions (right) on the week May 23-29.

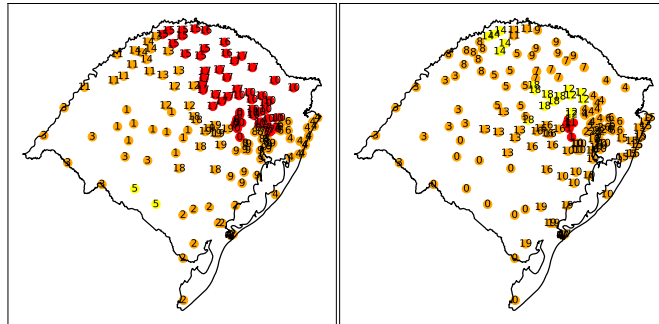

Figure 110: Flags assigned by our formula to the state's regions (left) and to the dynamic regions (right) on the week May 30 to June 5.

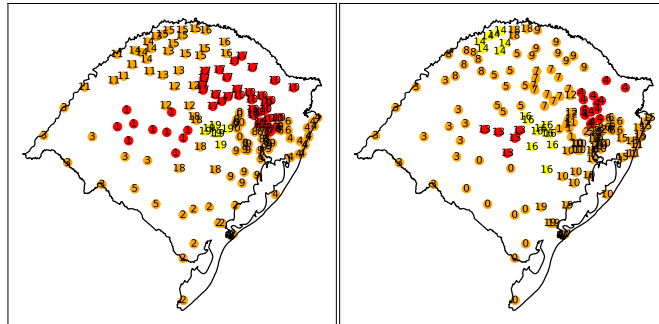

Figure 111: Flags assigned by our formula to the state's regions (left) and to the dynamic regions (right) on the week June 6-12.

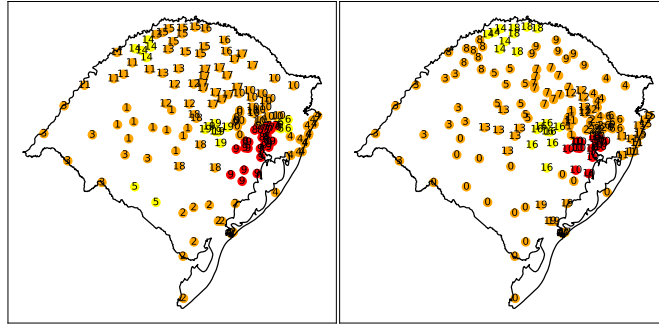

Figure 112: Flags assigned by our formula to the state's regions (left) and to the dynamic regions (right) on the week June 13-19.

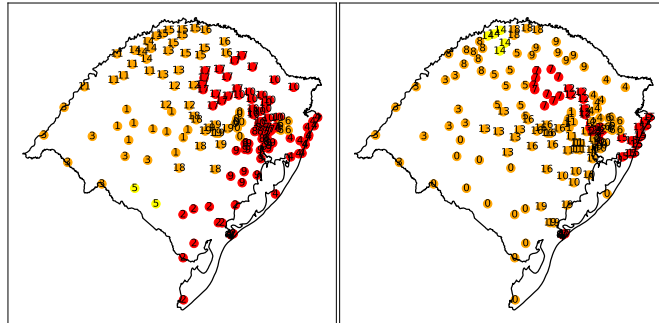

Figure 113: Flags assigned by our formula to the state's regions (left) and to the dynamic regions (right) on the week June 20-26.

### 3. SEIR model

The figures in this sections complement section 4 in the paper.

#### 3.1. Largest city from each cluster in section 1

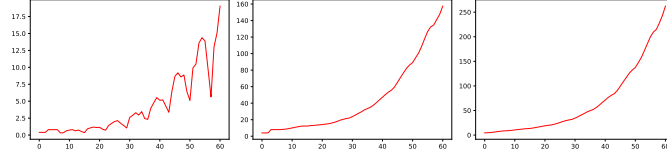

Figure 114: Gramado (center of cluster 1 in section 1, 62<sup>th</sup> largest city), number of new cases assuming the actual isolation data (left). Number of active cases (center). Overall number of cases (right).

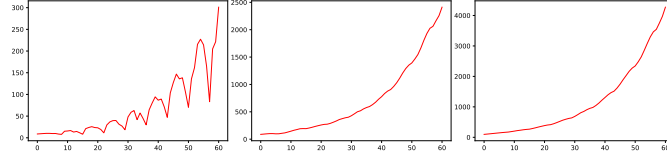

Figure 115: Santa Maria (center of cluster 2 in section 1, 5<sup>th</sup> largest city), number of new cases assuming the actual isolation data (left). Number of active cases (center). Overall number of cases (right).

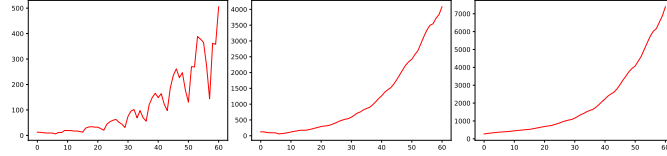

Figure 116: Porto Alegre (center of cluster 3 in section 1, largest city of the state), number of new cases assuming the actual isolation data (left). Number of active cases (center). Overall number of cases (right).

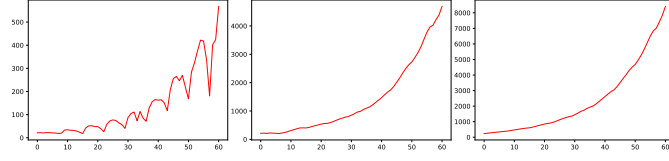

Figure 117: Passo Fundo (center of cluster 4 in section 1, 12<sup>th</sup> largest city), number of new cases assuming the actual isolation data (left). Number of active cases (center). Overall number of cases (right).

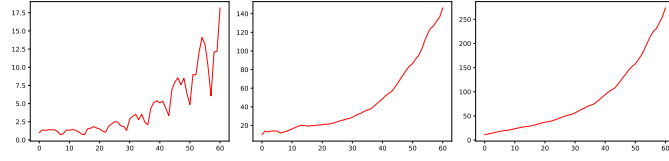

Figure 118: Osório (center of cluster 5 in section 1, 47<sup>th</sup> largest city), number of new cases assuming the actual isolation data (left). Number of active cases (center). Overall number of cases (right).

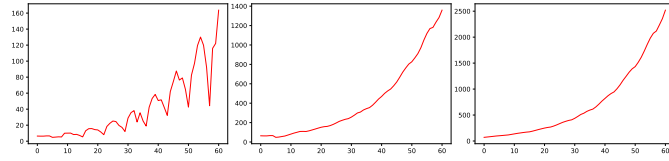

Figure 119: Santa Cruz do Sul (center of cluster 6 in section 1, 14<sup>th</sup> largest city), number of new cases assuming the actual isolation data (left). Number of active cases (center). Overall number of cases (right).

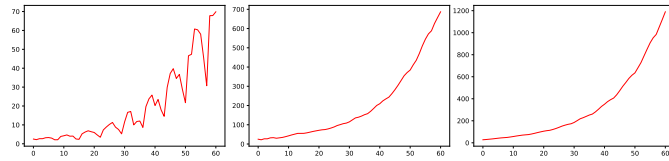

Figure 120: Pelotas (center of cluster 7 in section 1, 4<sup>th</sup> largest city), number of new cases assuming the actual isolation data (left). Number of active cases (center). Overall number of cases (right).

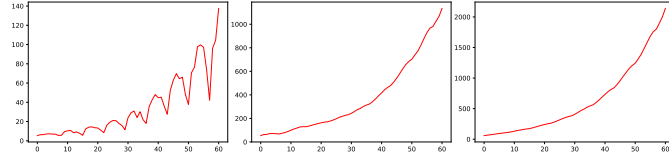

Figure 121: Novo Hamburgo (center of cluster 8 in section 1, 8<sup>th</sup> largest city), number of new cases assuming the actual isolation data (left). Number of active cases (center). Overall number of cases (right).

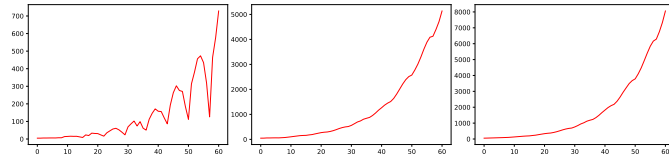

Figure 122: Caxias do Sul (center of cluster 9 in section 1, 2<sup>nd</sup> largest city), number of new cases assuming the actual isolation data (left). Number of active cases (center). Overall number of cases (right).

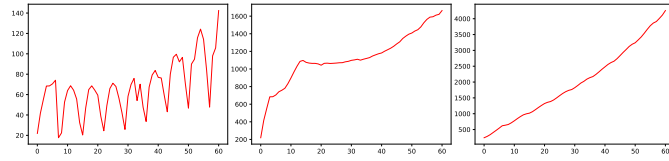

Figure 123: Lajeado (center of cluster 10 in section 1, 21<sup>th</sup> largest city), number of new cases assuming the actual isolation data (left). Number of active cases (center). Overall number of cases (right).

### 3.2. Other large cities

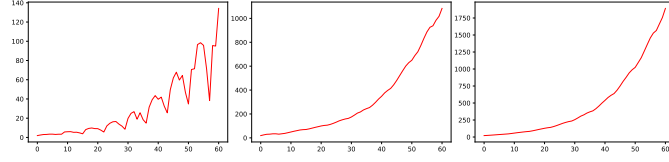

Figure 124: Canoas (member of cluster 3 in section 1, 3<sup>rd</sup> largest city), number of new cases assuming the actual isolation data (left). Number of active cases (center). Overall number of cases (right).

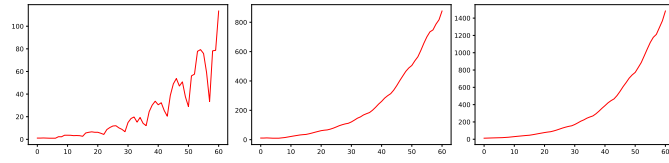

Figure 125: Gravataí (member of cluster 3 in section 1, 6<sup>th</sup> largest city), number of new cases assuming the actual isolation data (left). Number of active cases (center). Overall number of cases (right).

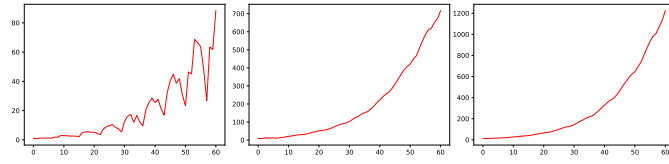

Figure 126: Viamão (member of cluster 3 in section 1, 7<sup>th</sup> largest city), number of new cases assuming the actual isolation data (left). Number of active cases (center). Overall number of cases (right).

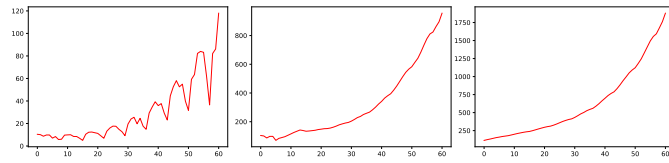

Figure 127: São Leopoldo (member of cluster 8 in section 1, 9<sup>th</sup> largest city), number of new cases assuming the actual isolation data (left). Number of active cases (center). Overall number of cases (right).

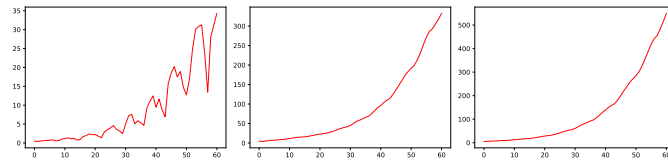

Figure 128: Rio Grande (member of cluster 7 in section 1,  $10^{th}$  largest city), number of new cases assuming the actual isolation data (left). Number of active cases (center). Overall number of cases (right).
